# Supplementary material for: Posterior Convergence of Nonparametric Binary and Poisson Regression Under Possible Misspecifications
Source: arXiv:2005.00234 source file (2020-05-01)
Supplement: Supplementary file 1 [file supp_gp.tex]

\setcounter{section}{0}
\setcounter{theorem}{0}

\begin{center}
{\LARGE\bf Supplementary Material}
\end{center}

\section{Preliminaries for ensuring posterior consistency under general set-up}
\label{sec:shalizi}

Following \ctn{Shalizi09} we consider a probability space $(\Omega,\mathcal F, P)$, 
and a sequence of random variables $y_1,y_2,\ldots$,   
taking values in some measurable space $(\Xi,\mathcal Y)$, whose
infinite-dimensional distribution is $P$. The natural filtration of this process is
$\sigma(\by_n)$. %where $\bY_n=(Y_1,Y_2,\ldots,Y_n)^T$.

We denote the distributions of processes adapted to $\sigma(\by_n)$ 
by $F_{\theta}$, where $\theta$ is associated with a measurable
space $(\Theta,\mathcal T)$, and is generally infinite-dimensional. 
For the sake of convenience, we assume, as in \ctn{Shalizi09}, that $P$
and all the $F_{\theta}$ are dominated by a common reference measure, with respective
densities $f_0$ and $f_{\theta}$. The usual assumptions that $P\in\Theta$ or even $P$ lies in the support 
of the prior on $\Theta$, are not required for Shalizi's result, rendering it very general indeed.

\subsection{Assumptions and theorems of Shalizi}
\label{subsec:assumptions_shalizi}

\begin{itemize}
\item[(S1)] Consider the following likelihood ratio:
\begin{equation}
R_n(\theta)=\frac{f_{\theta}(\bY_n)}{f_{\theta_0}(\bY_n)}.
\label{eq:R_n}
\end{equation}
Assume that $R_n(\theta)$ is $\sigma(\bY_n)\times \mathcal T$-measurable for all $n>0$.
\end{itemize}

\begin{itemize}
\item[(S2)] For every $\theta\in\Theta$, the KL-divergence rate
\begin{equation}
h(\theta)=\underset{n\rightarrow\infty}{\lim}~\frac{1}{n}E\left(\log\frac{f_{\theta_0}(\bY_n)}{f_{\theta}(\bY_n)}\right).
\label{eq:S3}
\end{equation}
exists (possibly being infinite) and is $\mathcal T$-measurable.
\end{itemize}

\begin{itemize}
\item[(S3)] For each $\theta\in\Theta$, the generalized or relative asymptotic equipartition property holds, and so,
almost surely,
\begin{equation*}
\underset{n\rightarrow\infty}{\lim}~\frac{1}{n}\log R_n(\theta)=-h(\theta).
\end{equation*}
\end{itemize}

\begin{itemize}
\item[(S4)] 
Let $I=\left\{\theta:h(\theta)=\infty\right\}$. 
The prior $\pi$ satisfies $\pi(I)<1$.
\end{itemize}

Following the notation of \ctn{Shalizi09}, for $A\subseteq\Theta$, let
\begin{align}
h\left(A\right)&=\underset{\theta\in A}{\mbox{ess~inf}}~h(\theta);\label{eq:h2}\\
J(\theta)&=h(\theta)-h(\Theta);\label{eq:J}\\
J(A)&=\underset{\theta\in A}{\mbox{ess~inf}}~J(\theta).\label{eq:J2}
\end{align}
\begin{itemize}
\item[(S5)] There exists a sequence of sets $\mathcal G_n\rightarrow\Theta$ as $n\rightarrow\infty$ 
such that: %along with $\pi(\mathcal G_T)>0$
\begin{enumerate}
\item[(1)]
\begin{equation}
\pi\left(\mathcal G_n\right)\geq 1-\alpha\exp\left(-\beta n\right),~\mbox{for some}~\alpha>0,~\beta>2h(\Theta);
\label{eq:S5_1}
\end{equation}
\item[(2)]The convergence in (S3) is uniform in $\theta$ over $\mathcal G_n\setminus I$.
\item[(3)] $h\left(\mathcal G_n\right)\rightarrow h\left(\Theta\right)$, as $n\rightarrow\infty$.
\end{enumerate}
\end{itemize}
For each measurable $A\subseteq\Theta$, for every $\delta>0$, there exists a random natural number $\tau(A,\delta)$
such that
\begin{equation}
n^{-1}\log\int_{A}R_n(\theta)\pi(\theta)d\theta
\leq \delta+\underset{n\rightarrow\infty}{\lim\sup}~n^{-1}
\log\int_{A}R_n(\theta)\pi(\theta)d\theta,
\label{eq:limsup_2}
\end{equation}
for all $n>\tau(A,\delta)$, provided 
$\underset{n\rightarrow\infty}{\lim\sup}~n^{-1}\log\pi\left(\mathbb I_A R_n\right)<\infty$.
%$\mathbb I_A$ denotes the indicator function of the set $A$.
Regarding this, the following assumption has been made by Shalizi:
\begin{itemize}
\item[(S6)] The sets $\mathcal G_n$ of (S5) can be chosen such that for every $\delta>0$, the inequality
$n>\tau(\mathcal G_n,\delta)$ holds almost surely for all sufficiently large $n$.
\end{itemize}
\begin{itemize}
\item[(S7)] The sets $\mathcal G_n$ of (S5) and (S6) can be chosen such that for any set $A$ with $\pi(A)>0$, 
\begin{equation}
h\left(\mathcal G_n\cap A\right)\rightarrow h\left(A\right),
\label{eq:S7}
\end{equation}
as $n\rightarrow\infty$.
\end{itemize}
Under the above assumptions, \ctn{Shalizi09} proved the following results.

\begin{theorem}[\ctn{Shalizi09}]
\label{theorem:shalizi1}
Consider assumptions (S1)--(S7) and any set $A\in\mathcal T$ with $\pi(A)>0$ and $h(A)>h(\Theta)$. Then,
\begin{equation*}
\underset{n\rightarrow\infty}{\lim}~\pi(A|\bY_n)=0~\mbox{almost surely},
%\label{eq:supp_post_conv1}
\end{equation*}
where $\pi(\cdot|\bY_n)$ denotes the posterior distribution of $\theta$ given $\bY_n$.
\end{theorem}

The rate of convergence of the log-posterior is given by the following result. 
\begin{theorem}[\ctn{Shalizi09}]
\label{theorem:shalizi2}
Consider assumptions (S1)--(S7) and any set $A\in\mathcal T$ with $\pi(A)>0$. If $\beta>2h(A)$, where
$\beta$ is given in (\ref{eq:S5_1}) under assumption (S5), or if $A\subset\cap_{k=n}^{\infty}\mathcal G_k$ for some $n$, then
\begin{equation*}
\underset{n\rightarrow\infty}{\lim}~\frac{1}{n}\log\pi(A|\bY_n)=-J(A),
%\label{eq:supp_post_conv2}
\end{equation*}
where $\pi(\cdot|\bY_n)$ denotes the posterior distribution of $\theta$ given $\bY_n$.
\end{theorem}
%We shall frequently make use of these theorems for our purpose.

\section{Verification of the assumptions of Shalizi for the Gaussian process model with normal errors}
\label{sec:verification}

\subsection{Verification of (S1)}
\label{subsec:S1}
note that
\begin{align}
f_{\theta}(\bY_n)&=\frac{1}{\left(\sigma\sqrt{2\pi}\right)^n}\exp\left\{-\frac{1}{2\sigma^2}\sum_{i=1}^n(Y_i-\eta(\bx_i))^2\right\};\label{eq:like1}\\
f_{\theta_0}(\bY_n)&=\frac{1}{\left(\sigma_0\sqrt{2\pi}\right)^n}\exp\left\{-\frac{1}{2\sigma^2_0}\sum_{i=1}^n(Y_i-\eta_0(\bx_i))^2\right\}.\label{eq:true_like1}
\end{align}
The equations (\ref{eq:like1}) and (\ref{eq:true_like1}) yield, in our case,
\begin{equation}
\frac{1}{n}\log R_n(\theta)=\log\left(\frac{\sigma_0}{\sigma}\right)+\frac{1}{2\sigma^2_0}\times\frac{1}{n}\sum_{i=1}^n\left(y_i-\eta_0(\bx_i)\right)^2
-\frac{1}{2\sigma^2}\times\frac{1}{n}\sum_{i=1}^n\left(y_i-\eta(\bx_i)\right)^2.
\label{eq:R1}
\end{equation}
We show that the right hand side of (\ref{eq:R1}), which we denote as $f(\by_n,\theta)$, is continuous in $(\by_n,\theta)$, which is sufficient to confirm measurability of $R_n(\theta)$.
Let $\|(\by_n,\theta)\|=\|\by_n\|+\|\theta\|$, where $\|\by_n\|$ is the Euclidean norm and $\|\theta\|=\|\eta\|+|\sigma|$, with
$\|\eta\|=\underset{\bx\in\mathcal X}{\sup}~|\eta(\bx)|$. Since $\mathcal X$ is compact and $\eta$ is almost surely continuous, it follows that $\|\eta\|<\infty$ almost surely.

Consider $\by_{n}=(y_{1},y_{2},\ldots,y_{n})^T$ %$\by_{2n}=(y_{21},y_{22},\ldots,y_{2n})^T$, $\theta_1$ and $\theta_2$. 
%such that, given $\varepsilon>0$, $\|(\by_{1n},\theta_1)-(\by_{2n},\theta_2)\|<\frac{\varepsilon}{c}$, for some finite $c>0$.
and $\boeta_{0n}=(\eta_0(\bx_1),\ldots,\eta_0(\bx_n))^T$. 
Then
\begin{equation}
\sum_{i=1}^n(y_{i}-\eta_0(\bx_i))^2=\by^T_n\by_n-2\by^T_n\boeta_{0n}+\boeta^T_{0n}\boeta_{0n}
\label{eq:cont2}
\end{equation}
is clearly continuous in $\by_n$.
%\begin{align}
%&\Bigg|\frac{1}{n}\sum_{i=1}^n(y_{1i}-\eta_0(\bx_i))^2-\frac{1}{n}\sum_{i=1}^n(y_{2i}-\eta_0(\bx_i))^2\Bigg |\notag\\%\label{eq:cont1}\\
%&=\frac{1}{n}\Bigg |\sum_{i=1}^n\left[(y_{1i}-y_{2i})\left\{(y_{1i}-\eta_0(\bx_i))+(y_{2i}-\eta_0(\bx_i))\right\}\right]\Bigg |\notag\\
%&\ \ \leq\|\by_{1n}-\by_{2n}\|\times\left(\frac{\|\by_{1n}-\boeta_{0n}\|}{n}+\frac{\|\by_{2n}-\boeta_{0n}\|}{n}\right).
%\label{eq:cont2}
%\end{align}
%Now note that for $j=1,2$, $\by_{jn}-\boeta_{0n}=\be_{jn}$, where $\be_{jn}=(\e_{j1},\ldots,\e_{jn})^T$ are the $iid$ Gaussian random errors with mean zero and variance $\sigma^2_0$.
%Since the elements of $\be_{jn}$ are almost surely finite, it follows that for $j=1,2$, $\frac{\|\by_{jn}-\boeta_{0n}\|}{n}=
%\sqrt{\sum_{i=1}^n\left(\frac{\e_{ji}}{n}\right)^2}$ is finite. 
%Let $c_1=\sum_{j=1}^2\sqrt{\sum_{i=1}^n\left(\frac{\e_{ji}}{n}\right)^2}$.
%Hence it follows from (\ref{eq:cont2}) that if $\|\by_{1n}-\by_{2n}\|<\frac{\varepsilon}{c_1}$, 
%then (\ref{eq:cont1}) is less than $\varepsilon$, which proves 
%Hence, continuity of the term $\frac{1}{n}\sum_{i=1}^n\left(y_i-\eta_0(\bx_i)\right)^2$ follows from (\ref{eq:cont2}).
%
Now note that 
\begin{equation}
\frac{1}{n}\sum_{i=1}^n(y_i-\eta(\bx_i))^2=\frac{1}{n}\sum_{i=1}^n(y_i-\eta_0(\bx_i))^2+\frac{1}{n}\sum_{i=1}^n(\eta(\bx_i)-\eta_0(\bx_i))^2
-\frac{2}{n}\sum_{i=1}^n(y_i-\eta_0(\bx_i))(\eta(\bx_i)-\eta_0(\bx_i)),
\label{eq:breakup2}
\end{equation}
where we have already proved continuity of the first term on the right hand side of (\ref{eq:breakup2}). %$\frac{1}{n}\sum_{i=1}^n(y_i-\eta_0(\bx_i))^2$.
To see continuity of $\frac{1}{n}\sum_{i=1}^n(\eta(\bx_i)-\eta_0(\bx_i))^2$ with respect to $\eta$, first consider any sequence $\left\{\eta_j:j=1,2,\ldots\right\}$ satisfying
$\|\eta_j-\tilde\eta\|\rightarrow 0$, as $j\rightarrow\infty$. Then
\begin{align}
&\Bigg|\frac{1}{n}\sum_{i=1}^n(\eta_j(\bx_i)-\eta_0(\bx_i))^2-\frac{1}{n}\sum_{i=1}^n(\tilde\eta(\bx_i)-\eta_0(\bx_i))^2\Bigg |\label{eq:cont3}\\
&\ \ \leq\frac{1}{n}\sum_{i=1}^n\left|\eta_j(\bx_i)-\tilde\eta(\bx_i)\right|\times\left|(\eta_j(\bx_i)-\eta_0(\bx_i))+(\tilde\eta(\bx_i)-\eta_0(\bx_i))\right|\notag\\
&\ \ \leq\|\eta_j-\tilde\eta\|\times\left[\|\eta_j-\eta_0\|+\|\tilde\eta-\eta_0\|\right]\notag\\
&\ \ \leq\|\eta_j-\tilde\eta\|\times\left[\|\eta_j-\tilde\eta\|+2\|\tilde\eta-\eta_0\|\right]\notag\\
&\ \ \rightarrow 0,~\mbox{as}~j\rightarrow\infty.
\label{eq:cont4}
\end{align}
%Due to continuity of $\eta_0$, $\eta_1$ and $\eta_2$, and compactness of $\mathcal X$, $\|\eta_j-\eta_0\|\leq \|\eta_j\|+\|\eta_0\|<\infty$, for $j=1,2$.
%Letting $c_2=\|\eta_1-\eta_0\|+\|\eta_2-\eta_0\|$, it follows that if $\|\eta_1-\eta_2\|<\frac{\varepsilon}{c_2}$, then (\ref{eq:cont3}) is less than $\varepsilon$,
This proves continuity of the second term of (\ref{eq:breakup2}). 

For the third term of (\ref{eq:breakup2}) we now prove that for any $\tilde \by\in\mathbb R^n$, and for any sequence 
$\left\{\by_j:j=1,2,\ldots\right\}$ (we denote the $i$-th component of $\by_j$ as $y_{ij}$) such that
$\|\by_j-\tilde\by\|\rightarrow 0$, as $j\rightarrow\infty$, and for any function $\tilde\eta$ associated with any sequence $\left\{\eta_j:j=1,2,\ldots\right\}$ satisfying
$\|\eta_j-\tilde\eta\|\rightarrow 0$, as $j\rightarrow\infty$, $\sum_{i=1}^n(y_{ij}-\eta_0(\bx_i))(\eta_j(\bx_i)-\eta_0(\bx_i))\rightarrow
\sum_{i=1}^n(\tilde y_i-\eta_0(\bx_i))(\tilde\eta(\bx_i)-\eta_0(\bx_i))$, as $j\rightarrow\infty$.
Indeed, observe that
\begin{align}
&\Bigg|\sum_{i=1}^n(y_{ij}-\eta_0(\bx_i))(\eta_j(\bx_i)-\eta_0(\bx_i))-\sum_{i=1}^n(\tilde y_i-\eta_0(\bx_i))(\tilde\eta(\bx_i)-\eta_0(\bx_i))\Bigg|\notag\\
&\qquad =\Bigg|\sum_{i=1}^n(y_{ij}-\tilde y_i)(\eta_j(\bx_i)-\tilde\eta(\bx_i))
+\sum_{i=1}^n(\tilde y_i-\eta_0(\bx_i))(\eta_j(\bx_i)-\tilde\eta(\bx_i))\notag\\
&\qquad\qquad +\sum_{i=1}^n(y_{ij}-\tilde y_i)(\tilde\eta(\bx_i)-\eta_0(\bx_i))\Bigg|\notag\\
&\qquad\leq n\|\by_j-\tilde\by\|\|\eta_j-\tilde\eta\|+%\left(\sqrt{\sum_{i=1}^n\epsilon^2_i}\right)
n\|\tilde\by-\boeta_{0n}\|\|\eta_j-\tilde\eta\|+n\|\by_j-\tilde\by\|\|\tilde\eta-\eta_0\|\notag\\
&\qquad\rightarrow 0,~\mbox{as}~\|\by_j-\tilde\by\|\rightarrow 0~\mbox{and}~\|\eta_j-\tilde\eta\|\rightarrow 0,~\mbox{as}~j\rightarrow\infty.\notag
\end{align}
Hence, $\sum_{i=1}^n(y_i-\eta_0(\bx_i))(\eta(\bx_i)-\eta_0(\bx_i))$ is continuous in $\by_n$ and $\eta$.
Continuity is clearly preserved if the above expression is divided by $\sigma$.

%\begin{align}
%&\Bigg|\frac{1}{n}\sum_{i=1}^n(y_i-\eta_0(\bx_i))(\eta_1(\bx_i)-\eta_0(\bx_i))-\frac{1}{n}\sum_{i=1}^n(y_i-\eta_0(\bx_i))(\eta_2(\bx_i)-\eta_0(\bx_i))\Bigg |\label{eq:cont5}\\
%& \ \ \Bigg|\frac{1}{n}\sum_{i=1}^n(y_i-\eta_0(\bx_i))(\eta_1(\bx_i)-\eta_2(\bx_i))\Bigg |\notag\\
%& \ \ \leq \left(\frac{1}{n}\sum_{i=1}^n\left|\e_i\right|\right)\times\|\eta_1-\eta_2\|,\label{eq:cont6}
%\end{align}
%where, for $i=1,\ldots,n$, $\e_i\stackrel{iid}{\sim}N\left(0,\sigma^2_0\right)$, are almost surely finite. Hence, (\ref{eq:cont6}) implies that, given $\e_1,\ldots,\e_n$, 
%$c_3=\frac{1}{n}\sum_{i=1}^n\left|\e_i\right|$ is a finite quantity. It follows that, if $\|\eta_1-\eta_2\|<\frac{\varepsilon}{c_3}$, then 
%(\ref{eq:cont5}) is less than $\varepsilon$.

Also, the first term of $f(\by_n,\theta)$, given by $\log\left(\frac{\sigma_0}{\sigma}\right)$, is clearly continuous
in $\sigma$. 
%where $\sigma>\xi>0$. That is, for given $\varepsilon>0$, there exists $c_4>0$ such that for $\sigma_1,\sigma_2$, both greater than $\xi$ and satisfying
%$|\sigma_1-\sigma_2|<\frac{\varepsilon}{c_4}$, $\left|\log\sigma_1-\log\sigma_2\right|<\varepsilon$. Hence it follows that for any 
%$\varepsilon>0$, if $c>\max\{c_1,c_2,c_3,c_4\}$, then $\|(\by_{1n},\theta_1)-(\by_{2n},\theta_2)\|<\frac{\varepsilon}{c}$ implies that
%$\left|f(\by_{1n},\theta_1)-f(\by_{1n},\theta_1)\right|<C\varepsilon$, for a finite $C>0$. 
Thus, continuity of $f(\by_n,\theta)$ with respect to $(\by_n,\theta)$ is guaranteed, so that (S1) holds.
Also observe that when the covariates are regarded as random, due to measurability of $\eta_0(\bX)$ assumed in (A4) and continuity of $\eta(\bx)$ in $\bx$.

\subsection{Verification of (S2) and proof of Lemma \ref{lemma:lemma1} for Gaussian errors}
\label{subsec:S2}
It follows from (\ref{eq:like1}) and (\ref{eq:true_like1}), that
\begin{equation}
\log\frac{f_{\theta_0}(\by_n)}{f_{\theta}(\by_n)}=n\log\left(\frac{\sigma}{\sigma_0}\right)-\frac{1}{2\sigma^2_0}\sum_{i=1}^n(y_i-\eta_0(\bx_i))^2+
\frac{1}{2\sigma^2}\sum_{i=1}^n(y_i-\eta(\bx_i))^2,
\label{eq:logratio1}
\end{equation}
so that
\begin{equation}
\frac{1}{n}E_{\theta_0}\left(\log\frac{f_{\theta_0}(\by_n)}{f_{\theta}(\by_n)}\right)=\log\left(\frac{\sigma}{\sigma_0}\right)-\frac{1}{2}
+\frac{\sigma^2_0}{2\sigma^2}+\frac{1}{2\sigma^2}\times\frac{1}{n}\sum_{i=1}^n\left(\eta(\bx_i)-\eta_0(\bx_i)\right)^2.
\label{eq:logratio2}
\end{equation}
By (A3), as $n\rightarrow\infty$,
\begin{equation}
\frac{1}{n}\sum_{i=1}^n\left(\eta(\bx_i)-\eta_0(\bx_i)\right)^2\rightarrow E_\bX\left[\eta(\bX)-\eta_0(\bX)\right]^2
=\int_{\mathcal X}\left[\eta(\bX)-\eta_0(\bX)\right]^2dQ.
\label{eq:slln1}
\end{equation}
Hence,
\begin{equation}
\frac{1}{n}E_{\theta_0}\left(\log\frac{f_{\theta_0}(\by_n)}{f_{\theta}(\by_n)}\right)\rightarrow \log\left(\frac{\sigma}{\sigma_0}\right)-\frac{1}{2}
+\frac{\sigma^2_0}{2\sigma^2}+\frac{1}{2\sigma^2}E_\bX\left[\eta(\bX)-\eta_0(\bX)\right]^2,~\mbox{as}~n\rightarrow\infty.
\label{eq:logratio3}
\end{equation}
We let
\begin{equation*}
h(\theta)=\log\left(\frac{\sigma}{\sigma_0}\right)-\frac{1}{2}+\frac{\sigma^2_0}{2\sigma^2}+\frac{1}{2\sigma^2}E_\bX\left[\eta(\bX)-\eta_0(\bX)\right]^2.
%\label{eq:h}
\end{equation*}

\subsection{Verification of (S3) and proof of Theorem \ref{theorem:theorem1} for Gaussian errors}
\label{subsec:S3}

By SLLN, as $n\rightarrow\infty$,
\begin{equation}
\frac{1}{n}\sum_{i=1}^n\left(y_i-\eta_0(\bx_i)\right)^2\stackrel{a.s.}{\longrightarrow}\sigma^2_0,
\label{eq:slln2}
\end{equation}
where $``\stackrel{a.s.}{\longrightarrow}"$ denotes convergence almost surely.
Also,
\begin{align}
\frac{1}{n}\sum_{i=1}^n\left(y_i-\eta(\bx_i)\right)^2 &=\frac{1}{n}\sum_{i=1}^n\left(y_i-\eta_0(\bx_i)\right)^2+\frac{1}{n}\sum_{i=1}^n\left(\eta(\bx_i)-\eta_0(\bx_i)\right)^2\notag\\
&\qquad\qquad+\frac{2}{n}\sum_{i=1}^n\left(y_i-\eta_0(\bx_i)\right)\left(\eta_0(\bx_i)-\eta(\bx_i)\right).
\label{eq:breakup1}
\end{align}
By (\ref{eq:slln2}) the first term on the right hand side of (\ref{eq:breakup1}) converges almost surely to $\sigma^2_0$. The second term converges to 
$E_{\bX}\left[\eta(\bX)-\eta_0(\bX)\right]^2$ and the
third term converges almost surely to zero by Kolmogorov's SLLN for independent random variables, noting that $y_i-\eta_0(\bx_i)=\e_i$ are independent zero mean random variables
and $\sum_{i=1}^{\infty}i^{-2}Var\left((y_i-\eta_0(\bx_i)(\eta_0(\bx_i)-\eta(\bx_i))\right)=\sigma^2_0\sum_{i=1}^{\infty}i^{-2}\left(\eta_0(\bx_i)-\eta(\bx_i)\right)^2\leq
\sigma^2_0\|\eta-\eta_0\|^2\sum_{i=1}^{\infty}i^{-2}<\infty$. %is independent of $\bX_i$ and hence of $\eta_0(\bx_i)-\eta(\bx_i)$, for $i=1,\ldots,n$.
Hence, letting $n\rightarrow\infty$ in (\ref{eq:R1}), it follows that
\begin{equation}
\frac{1}{n}\log R_n(\theta)\stackrel{a.s.}{\longrightarrow}\log\left(\frac{\sigma_0}{\sigma}\right)+\frac{1}{2}-\frac{\sigma^2_0}{2\sigma^2}
-\frac{1}{2\sigma^2}E_{\bX}\left[\eta(\bX)-\eta_0(\bX)\right]^2=-h(\theta).
\label{eq:R2}
\end{equation}
The above results of course remain the same if the covariates are assumed to be random.

\subsection{Verification of (S4)}
\label{subsec:S4}

Note that $h(\theta)\leq\log\left(\frac{\sigma}{\sigma_0}\right)-\frac{1}{2}+\frac{\sigma^2_0}{2\sigma^2}+\frac{\|\eta-\eta_0\|^2}{2\sigma^2}$, where
$0<\sigma<\infty$ and $0<\|\eta-\eta_0\|<\infty$ with prior probability one. Hence, $h(\theta)<\infty$ with probability one, showing that (S4) holds.
\begin{comment}
By (A5), 
\begin{equation}
\pi\left(\sigma=\infty\right)=0. 
\label{eq:sigma_prior}
\end{equation}
Also, since $\|\eta\|<\infty$ almost surely, and $\|\eta_0\|<\infty$ by (A4), it follows that
\begin{equation}
\pi\left(\|\eta-\eta_0\|=\infty\right)=0.
\label{eq:gp_finite}
\end{equation}
Now, in (\ref{eq:h}) note that $E_\bX\left[\eta(\bX)-\eta_0(\bX)\right]^2\leq \|\eta-\eta_0\|^2$, so that 
\begin{align}
\pi\left(h(\theta)=\infty\right)&\leq\pi\left(\left\{\sigma=\infty\right\}\cup\left\{\|\eta-\eta_0\|=\infty\right\}\right)\notag\\
&\leq\pi\left(\sigma=\infty\right)+\pi\left(\|\eta-\eta_0\|=\infty\right)\notag\\
&=0,~\mbox{due to (\ref{eq:sigma_prior}) and (\ref{eq:gp_finite})}.\notag
\end{align}
Hence, (S4) holds.
\end{comment}

\subsection{Verification of (S5)}
\label{subsec:S5}

\subsubsection{Verification of (S5) (1)}
\label{subsubsec:S5_1}

%Let $\sigma^2_{\mathcal X}=\underset{\bx\in\mathcal X}{\sup}~E\left[\eta(\bx)-\mu(\bx)\right]^2$ and for $j=1,\ldots,d$,
%$\sigma^2_{j,\mathcal X}=\underset{\bx\in\mathcal X}{\sup}~E\left[\eta'_j(\bx)-\mu'_j(\bx)\right]^2$, where $\mu'_j$ stands for the $j$-th partial derivative of $\mu$. 
%Note that, due to compactness of $\mathcal X$,
%these quantities are finite.

%By (A5), there exists $\alpha\in (0,1)$ and $\beta>0$ such that $\alpha\beta>2h(\Theta)$. Now, for any real-valued function $f$ on $\mathcal X$, let us define 
%$\|f\|_0=\underset{\bx\in\mathcal X}{\sup}~f(\bx)$. 
%With this, 
Recall that
\begin{align}
%\mathcal G_n&=\left\{\left(\eta,\sigma\right):\|\eta-\mu\|\leq\sqrt{2\beta\sigma^2_{\mathcal X} n}+E\|\eta-\mu\|,\right.\notag\\
%&\left.\|\eta'_j-\mu'_j\|\leq\sqrt{2\beta\sigma^2_{j,\mathcal X} n}+E\|\eta'_j-\mu'_j\|;j=1,\ldots,d,n^{-\frac{1}{2q}}\leq\sigma\leq\exp\left(\beta n\right)\right\},
\mathcal G_n&=\left\{\left(\eta,\sigma\right):\|\eta\|\leq\exp(\sqrt{\beta n}),\exp(-\sqrt{\beta n})\leq\sigma\leq\exp(\sqrt{\beta n}),
\|\eta'_j\|\leq\exp(\sqrt{\beta n});j=1,\ldots,d\right\}.\notag
%\label{eq:G}
\end{align}
Then $\mathcal G_n\rightarrow\Theta$, as $n\rightarrow\infty$.
Now note that
\begin{align}
&\pi(\mathcal G_n)=\pi\left(\|\eta\|\leq\exp(\sqrt{\beta n}),\exp(-\sqrt{\beta n})\leq\sigma\leq\exp(\sqrt{\beta n})\right)\notag\\
%&\ \ -\pi\left(\left\{\|\eta-\mu\|\leq\sqrt{2\beta\sigma^2_{\mathcal X} n}+E\|\eta-\mu\|,\|\eta'_j-\mu'_j\|\leq\sqrt{2\beta\sigma^2_{j,\mathcal X} n}
%+E\|\eta'_j-\mu'_j\|;j=1,\ldots,d\right\}^c\right)\notag\\
&\ \ -\pi\left(\left\{\|\eta'_j\|\leq\exp(\sqrt{\beta n});j=1,\ldots,d\right\}^c\right)\notag\\
%&=\pi\left(n^{-\frac{1}{2q}}\leq\sigma\leq\exp\left(\beta n\right)\right)\notag\\
%&\ \ -\pi\left(\left\{\|\eta-\mu\|>\sqrt{2\beta\sigma^2_{\mathcal X} n}+E\|\eta-\mu\|\right\}\bigcup\left[\bigcup_{j=1}^d\left\{\|\eta'_j-\mu'_j\|>\sqrt{2\beta\sigma^2_{j,\mathcal X} n}
%+E\|\eta'_j-\mu'_j\|\right\}\right]\right)\notag\\
%&=\pi\left(\frac{\|\eta\|}{\sigma}\leq\beta^{\frac{1}{2q}}n^{\frac{1}{2q}},n^{-\frac{1}{2q}}\leq\sigma\leq\beta n\right)\notag\\
%&\ \ -\pi\left(\left\{\|\eta-\mu\|>\sqrt{2\beta\sigma^2_{\mathcal X} n}+E\|\eta-\mu\|\right\}\bigcup\left[\bigcup_{j=1}^d\left\{\|\eta'_j-\mu'_j\|>\sqrt{2\beta\sigma^2_{j,\mathcal X} n}
%+E\|\eta'_j-\mu'_j\|\right\}\right]\right)\notag\\
&=\pi\left(\|\eta\|\leq\exp(\sqrt{\beta n}),\exp(-\sqrt{\beta n})\leq\sigma\leq\exp(\sqrt{\beta n})\right)\notag\\
&\ \ -\pi\left(\bigcup_{j=1}^d\left\{\|\eta'_j\|>\exp(\sqrt{\beta n})\right\}\right)\notag\\
%&\ \ \geq\pi\left(n^{-\frac{1}{2q}}\leq\sigma\leq\exp\left(\beta n\right)\right)-\pi\left(\|\eta-\mu\|>\sqrt{2\beta\sigma^2_{\mathcal X} n}+E\|\eta-\mu\|\right)\notag\\
%&\ \ \  \ -\sum_{j=1}^d\pi\left(\|\eta'_j-\mu'_j\|>\sqrt{2\beta\sigma^2_{j,\mathcal X} n}+E\|\eta'_j-\mu'_j\|\right).
& \geq 1-\pi\left(\|\eta\|>\exp(\sqrt{\beta n})\right)-\pi\left(\left\{\exp(-\sqrt{\beta n})\leq\sigma\leq\exp(\sqrt{\beta n})\right\}^c\right)\notag\\
&\ \ \  \ -\sum_{j=1}^d\pi\left(\|\eta'_j\|>\exp(\sqrt{\beta n})\right)\notag\\
&\geq 1-(c_{\eta}+c_{\sigma}+\sum_{j=1}^dc_{\eta^\prime_j})\exp(-\beta n),
\label{eq:s5_1}
\end{align}
by the Borell-TIS inequality and (A5). 
In other words, (S5) (1) holds.

\subsubsection{Verification of (S5) (2)}
\label{subsubsec:S5_2}

We now show that (S5) (2), namely, convergence in (S3) is uniform in $\theta$ over $\mathcal G_n\setminus I$ holds. First note that $I=\emptyset$ in our case, so that
$\mathcal G_n\setminus I=\mathcal G_n$. 

To proceed further, we show that $\mathcal G_n$ is compact.
Note that $\mathcal G_n=\mathcal G_{n,\eta}\times \mathcal G_{n,\sigma}$, where
\begin{align}
%\mathcal G_{n,\eta}&=\left\{\eta:\|\eta-\mu\|\leq\sqrt{2\beta\sigma^2_{\mathcal X} n}+E\|\eta-\mu\|,\right.\notag\\
\mathcal G_{n,\eta}&=\left\{\eta:\|\eta\|\leq\exp(\sqrt{\beta n}),~\|\eta'_j\|\leq\exp(\sqrt{\beta n});j=1,\ldots,d\right\}\notag
%\label{eq:G_eta}
\end{align}
and
\begin{equation*}
\mathcal G_{n,\sigma}=\left\{\sigma:\exp(-\sqrt{\beta n})\leq\sigma\leq\exp(\sqrt{\beta n})\right\}.
%\label{eq:G_sigma}
\end{equation*}
%Since $\mathcal G_n$ is closed, and closed subsets of compact sets are compact, it is sufficient to prove that $\mathcal G_{n,\eta}\times \mathcal G_{n,\sigma}$ is compact.
Since $\mathcal G_{n,\sigma}$ is compact and products of compact sets is compact, it is enough to prove compactness of $\mathcal G_{n,\eta}$.
We use the Arzela-Ascoli lemma to prove that $\mathcal G_{n,\eta}$ is compact for each $n\geq 1$. 
In other words, $\mathcal G_{n,\eta}$ is compact if and only if it is closed,
bounded and equicontinuous. By boundedness we mean $|\eta(\bx)|<M$ for each $\bx\in\mathcal X$ and for each $\eta\in\mathcal G_{n,\eta}$. Equicontinuity entails
that for any $\epsilon>0$, there exists $\delta>0$ which depends only on $\epsilon$ such that $|\eta(\bx_1)-\eta(\bx_2)|<\epsilon$ whenever $\|\bx_1-\bx_2\|<\delta$,
for all $\eta\in\mathcal G_{n,\eta}$. Closedness and boundedness are obvious from the definition of $\mathcal G_{n,\eta}$. Equicontinuity follows from the fact that
the elements of $\mathcal G_{n,\eta}$ are Lipschitz continuous thanks to boundedness of the partial derivatives. Thus, $\mathcal G_{n,\eta}$, and hence $\mathcal G_n$ is compact.

Since $\mathcal G_n$ is compact for all $n\geq 1$, uniform convergence as required will be proven if we can show that $\frac{1}{n}\log R_n(\theta)+h(\theta)$ is 
stochastically equicontinuous almost surely in $\theta\in\mathcal G$ for any 
$\mathcal G\in\left\{\mathcal G_n:n=1,2,\ldots\right\}$ and $\frac{1}{n}\log R_n(\theta)+h(\theta)\rightarrow 0$, almost surely, for all $\theta\in\mathcal G$
(see \ctn{Newey91}, \ctn{Billingsley13}) for the general theory of uniform convergence in compact sets under stochastic equicontinuity). 
Since, in the context of (S3) we have already shown almost sure pointwise convergence of $\frac{1}{n}\log R_n(\theta)$ to $-h(\theta)$, it is enough to verify stochastic
equicontinuity of $\frac{1}{n}\log R_n(\theta)+h(\theta)$ in $\mathcal G\in\left\{\mathcal G_n:n=1,2,\ldots\right\}$.

Stochastic equicontinuity usually follows easily if one can prove that the function concerned is almost surely Lipschitz continuous.
Recall
from (\ref{eq:R1}), (\ref{eq:cont2}), (\ref{eq:breakup2}) and (\ref{eq:cont4}) that if the term $\frac{1}{n}\sum_{i=1}^n(y_i-\eta_0(\bx_i))(\eta(\bx_i)-\eta_0(\bx_i))$
can be proved Lipschitz continuous in $\eta\in\mathcal G$, then $\frac{1}{n}\log R_n(\theta)$ is Lipschitz for $\eta\in\mathcal G$. Also, if $E_{\bX}\left[\eta(\bX)-\eta_0(\bX)\right]^2$
is Lipschitz in $\eta$, then it would follow from (\ref{eq:h}) that $h(\theta)$ is Lipschitz for $\eta\in\mathcal G$. Since sum of Lipschitz functions is Lipschitz, this would imply
that $\frac{1}{n}\log R_n(\theta)+h(\theta)$ is Lipschitz in $\eta\in\mathcal G$. Since the first derivative of $\frac{1}{n}\log R_n(\theta)+h(\theta)$
with respect to $\sigma$ is bounded (as $\sigma$ is bounded in $\mathcal G$), it would then follow that $\frac{1}{n}\log R_n(\theta)+h(\theta)$ is Lipschitz for $\theta\in\mathcal G$. 
Hence, to see that $\frac{1}{n}\sum_{i=1}^n(y_i-\eta_0(\bx_i))(\eta(\bx_i)-\eta_0(\bx_i))$ is almost surely Lipschitz in $\eta\in\mathcal G$, note that for any $\eta_1,\eta_2\in\mathcal G$,
\begin{align}
&\left|\frac{1}{n}\sum_{i=1}^n(y_i-\eta_0(\bx_i))(\eta_1(\bx_i)-\eta_0(\bx_i))-\frac{1}{n}\sum_{i=1}^n(y_i-\eta_0(\bx_i))(\eta_2(\bx_i)-\eta_0(\bx_i))\right|\notag\\
&\qquad\qquad\leq\|\eta_1-\eta_2\|\times\frac{1}{n}\sum_{i=1}^n\left|y_i-\eta(\bx_i)\right|.\notag
\end{align}
Hence, $\frac{1}{n}\sum_{i=1}^n(y_i-\eta_0(\bx_i))(\eta(\bx_i)-\eta_0(\bx_i)$ is Lipschitz in $\eta$ and since $\frac{1}{n}\sum_{i=1}^n\left|y_i-\eta(\bx_i)\right|\rightarrow
E_{\theta_0}\left|y_1-\eta(\bx_1)\right|\leq E_{\theta_0}\left|y_1-\eta_0(\bx_1)\right|+\left|\eta_0(\bx_1)-\eta(\bx_1)\right|<\infty$ as $n\rightarrow\infty$, stochastic equicontinuity follows.

That $E_{\bX}\left[\eta(\bX)-\eta_0(\bX)\right]^2$ is also Lipschitz in $\mathcal G$ can be seen from the fact that for $\eta_1,\eta_2\in\mathcal G$,
\begin{equation*}
\left|E_{\bX}\left[\eta_1(\bX)-\eta_0(\bX)\right]^2-E_{\bX}\left[\eta_2(\bX)-\eta_0(\bX)\right]^2\right|
\leq\|\eta_1-\eta_2\|\times\left[\|\eta_1\|+\|\eta_2\|+2\|\eta_0\|\right],
\end{equation*}
where $\|\eta_0\|<\kappa_0$ by (A4) and for $j=1,2$, %$\|\eta_j\|\leq\|\eta_j-\mu\|+\|\mu\|\leq\sqrt{2\beta\sigma^2_{\mathcal X}m}+E\|\eta_j-\mu\|+\|\mu\|$, 
$\|\eta_j\|\leq \exp(\sqrt{\beta m})$,
where $\mathcal G=\mathcal G_m$, for $m\geq 1$.

\subsubsection{Verification of (S5) (3)}
\label{subsubsec:S5_3}

We now verify (S5) (3). For our purpose, let us show that $h(\theta)$ is continuous in $\theta$. Continuity will easily follow if we can show that $E_{\bX}\left[\eta(\bX)-\eta_0(\bX)\right]^2$
is continuous in $\eta$. As before, let $\eta_j$ be a sequence of functions converging to $\tilde\eta$ in the sense $\|\eta_j-\tilde\eta\|\rightarrow 0$ as $j\rightarrow\infty$.
Then, since $\left|E_{\bX}\left[\eta_j(\bX)-\eta_0(\bX)\right]^2-E_{\bX}\left[\tilde\eta(\bX)-\eta_0(\bX)\right]^2\right|
\leq \|\eta_j-\tilde\eta\|\left[\|\eta_j-\tilde\eta\|+2\|\tilde\eta-\eta_0\|\right]
\rightarrow 0$ as $j\rightarrow\infty$, continuity follows. Hence, continuity of $h(\theta)$, compactness of $\mathcal G_n$, along with its non-decreasing nature with respect to $n$ implies that 
$h\left(\mathcal G_n\right)\rightarrow h(\Theta)$, as $n\rightarrow\infty$.

\subsection{Verification of (S6) and proof of Theorem \ref{theorem:theorem3} for Gaussian errors}
\label{subsec:S6}

Observe that 
\begin{align}
\frac{1}{n}\log R_n(\theta)+h(\theta)&=\left[\frac{1}{2\sigma^2_0}\times\frac{1}{n}\sum_{i=1}^n\left(y_i-\eta_0(\bx_i)\right)^2-\frac{1}{2}\right]
+\left[\frac{1}{2\sigma^2}\times\frac{1}{n}\sum_{i=1}^n\left(y_i-\eta_0(\bx_i)\right)^2-\frac{\sigma^2_0}{2\sigma^2}\right]\notag\\
&\qquad+\left[\frac{1}{2\sigma^2}\times\frac{1}{n}\sum_{i=1}^n\left(\eta(\bx_i)-\eta_0(\bx_i)\right)^2-\frac{1}{2\sigma^2}E_{\bX}\left(\eta(\bX)-\eta_0(\bX)\right)^2\right]\notag\\
&\qquad+\left[\frac{1}{\sigma^2}\times\frac{1}{n}\sum_{i=1}^n\left(y_i-\eta_0(\bx_i)\right)\left(\eta(\bx_i)-\eta_0(\bx_i)\right)\right].
\label{eq:s5_5}
\end{align}
Let $\kappa_1=\kappa-h(\Theta)$. Then it follows from (\ref{eq:s5_5}) that for all $\theta\in\mathcal G$, we have
\begin{align}
&P\left(\left|\frac{1}{n}\log R_n(\theta)+h(\theta)\right|>\kappa_1\right)\notag\\
&\leq P\left(\left|\frac{1}{2\sigma^2_0}\times\frac{1}{n}\sum_{i=1}^n\left(y_i-\eta_0(\bx_i)\right)^2-\frac{1}{2}\right|>\frac{\kappa_1}{4}\right)
+P\left(\left|\frac{1}{2\sigma^2}\times\frac{1}{n}\sum_{i=1}^n\left(y_i-\eta_0(\bx_i)\right)^2-\frac{\sigma^2_0}{2\sigma^2}\right|>\frac{\kappa_1}{4}\right)\notag\\
&\qquad+P\left(\left|\frac{1}{2\sigma^2}\times\frac{1}{n}\sum_{i=1}^n\left(\eta(\bx_i)-\eta_0(\bx_i)\right)^2
-\frac{1}{2\sigma^2}E_{\bX}\left(\eta(\bX)-\eta_0(\bX)\right)^2\right|>\frac{\kappa_1}{4}\right)\notag\\
&\qquad+P\left(\left|\frac{1}{\sigma^2}\times\frac{1}{n}\sum_{i=1}^n\left(y_i-\eta_0(\bx_i)\right)\left(\eta(\bx_i)-\eta_0(\bx_i)\right)\right|>\frac{\kappa_1}{4}\right).
\label{eq:s5_6}
\end{align}

Note that $\sum_{i=1}^n\left(\frac{y_i-\eta_0(\bx_i)}{\sigma_0}\right)^2=\bz^T_n\bz_n$, %\sim\chi^2_n$, using Markov's inequality similarly as in \ctn{Choi07}, 
where $\bz_n\sim N_n\left(\bzero_n,\bI_n\right)$, the $n$-dimensional normal distribution with mean $\bzero_n=(0,0,\ldots,0)^T$ and covariance matrix $\bI_n$, the identity matrix. 
Using the Hanson-Wright inequality we bound the
first term of the right hand side of (\ref{eq:s5_6}) as follows:
\begin{align}
&P\left(\left|\frac{1}{2\sigma^2_0}\times\frac{1}{n}\sum_{i=1}^n\left(y_i-\eta_0(\bx_i)\right)^2-\frac{1}{2}\right|>\frac{\kappa_1}{4}\right)\notag\\
&\qquad=P\left(\left|\bz^T_n\bz_n-n\right|>\frac{n\kappa_1}{2}\right)\notag\\
&\qquad\leq 2\exp\left(-n\min\left\{\frac{\kappa^2_1}{16c_0},\frac{\kappa_1}{4c_0}\right\}\right),
%&=P\left(\sum_{i=1}^n\left(\frac{y_i-\eta_0(\bx_i)}{\sigma_0}\right)^2>n\left(1+\frac{\kappa_1}{2}\right)\right)
%+P\left(\sum_{i=1}^n\left(\frac{y_i-\eta_0(\bx_i)}{\sigma_0}\right)^2<n\left(1-\frac{\kappa_1}{2}\right)\right)\notag\\
%&\leq\exp\left\{-n\left(\frac{\kappa^2_1}{16}-\frac{\kappa^3_1}{48}\right)\right\}+\exp\left\{-n\left(\frac{\kappa^2_1}{16}\right)\right\}.
\label{eq:s5_7}
\end{align}
where $c_0>0$ is a constant.
It follows from (\ref{eq:s5_7}) that
\begin{equation}
\int_{\mathcal S^c}P\left(\left|\frac{1}{2\sigma^2_0}\times\frac{1}{n}\sum_{i=1}^n\left(y_i-\eta_0(\bx_i)\right)^2-\frac{1}{2}\right|>\frac{\kappa_1}{4}\right)d\pi(\theta)
\leq 2\exp\left(-n\min\left\{\frac{\kappa^2_1}{16c_0},\frac{\kappa_1}{4c_0}\right\}\right).
\label{eq:s5_7_int}
\end{equation}

In almost the same way as in (\ref{eq:s5_7}), the second term of the right hand side of (\ref{eq:s5_6}) can be bounded as:
\begin{align}
&P\left(\left|\frac{1}{2\sigma^2}\times\frac{1}{n}\sum_{i=1}^n\left(y_i-\eta_0(\bx_i)\right)^2-\frac{\sigma^2_0}{2\sigma^2}\right|>\frac{\kappa_1}{4}\right)\notag\\
&\qquad=P\left(\left|\bz^T_n\bz_n-n\right|>\frac{n\kappa_1\sigma^2}{2\sigma^2_0}\right)\notag\\
&\qquad\leq 2\exp\left(-n\min\left\{\frac{\kappa^2_1\sigma^4}{16c_0\sigma^4_0},\frac{\kappa_1\sigma^2}{4c_0\sigma^2_0}\right\}\right).
%&=P\left(\left|\frac{1}{n}\sum_{i=1}^n\left(y_i-\eta_0(\bx_i)\right)^2-1\right|>\frac{\kappa_1\sigma^2}{2\sigma^2_0}\right)\notag\\
%&\leq P\left(\left|\frac{1}{n}\sum_{i=1}^n\left(y_i-\eta_0(\bx_i)\right)^2-1\right|>\frac{\delta\xi^2}{2\sigma^2_0}\right)\notag\\
%&=P\left(\sum_{i=1}^n\left(\frac{y_i-\eta_0(\bx_i)}{\sigma_0}\right)^2>n\left(1+\frac{\kappa_1\sigma^2}{2\sigma^2_0}\right)\right)
%+P\left(\sum_{i=1}^n\left(\frac{y_i-\eta_0(\bx_i)}{\sigma_0}\right)^2<n\left(1-\frac{\kappa_1\sigma^2}{2\sigma^2_0}\right)\right)\notag\\
%&\leq\exp\left\{-n\left(\frac{\kappa^2_1\sigma^4}{16\sigma^4_0}-\frac{\kappa^3_1\sigma^6}{48\sigma^6_0}\right)\right\}
%+\exp\left\{-n\left(\frac{\kappa^2_1\sigma^4}{16\sigma^4_0}\right)\right\}.
\label{eq:s5_8}
\end{align}
Now
\begin{align}
&\int_{\mathcal S^c}P\left(\left|\frac{1}{2\sigma^2}\times\frac{1}{n}\sum_{i=1}^n\left(y_i-\eta_0(\bx_i)\right)^2-\frac{\sigma^2_0}{2\sigma^2}\right|>\frac{\kappa_1}{4}\right)d\pi(\theta)\notag\\
&\leq \int_{\mathcal G_n}2\exp\left(-n\min\left\{\frac{\kappa^2_1\sigma^4}{16c_0\sigma^4_0},\frac{\kappa_1\sigma^2}{4c_0\sigma^2_0}\right\}\right)\pi(\sigma^2)d\sigma^2\notag\\
&\qquad+\int_{\mathcal G^c_n}2\exp\left(-n\min\left\{\frac{\kappa^2_1\sigma^4}{16c_0\sigma^4_0},\frac{\kappa_1\sigma^2}{4c_0\sigma^2_0}\right\}\right)\pi(\theta)d\theta\notag\\
&\leq \int_{\mathcal G_n}2\exp\left(-n\min\left\{\frac{\kappa^2_1\sigma^4}{16c_0\sigma^4_0},\frac{\kappa_1\sigma^2}{4c_0\sigma^2_0}\right\}\right)\pi(\sigma^2)d\sigma^2
+2\pi(\mathcal G^c_n)\notag\\
&\leq \int_{\mathcal G_n\cap\left\{\frac{\kappa_1\sigma^2}{4\sigma^2_0}\leq 1\right\}}2\exp\left(-n\min\left\{\frac{\kappa^2_1\sigma^4}{16c_0\sigma^4_0},\frac{\kappa_1\sigma^2}{4c_0\sigma^2_0}\right\}\right)\pi(\sigma^2)d\sigma^2\notag\\
&\qquad+\int_{\mathcal G_n\cap\left\{\frac{\kappa_1\sigma^2}{4\sigma^2_0}> 1\right\}}2\exp\left(-n\min\left\{\frac{\kappa^2_1\sigma^4}{16c_0\sigma^4_0},\frac{\kappa_1\sigma^2}{4c_0\sigma^2_0}\right\}\right)\pi(\sigma^2)d\sigma^2+2\pi(\mathcal G^c_n)\notag\\
&=\int_{\mathcal G_n\cap\left\{\frac{\kappa_1\sigma^2}{4\sigma^2_0}\leq 1\right\}}2\exp\left(-n\frac{\kappa^2_1\sigma^4}{16c_0\sigma^4_0}\right)\pi(\sigma^2)d\sigma^2\notag\\
&\qquad+\int_{\mathcal G_n\cap\left\{\frac{\kappa_1\sigma^2}{4\sigma^2_0}> 1\right\}}2\exp\left(-n\frac{\kappa_1\sigma^2}{4c_0\sigma^2_0}\right)\pi(\sigma^2)d\sigma^2+2\pi(\mathcal G^c_n)\notag\\
&\leq\int_{\exp(-2\sqrt{\beta n})}^{\exp(2\sqrt{\beta n})}2\exp\left(-n\frac{\kappa^2_1\sigma^4}{16c_0\sigma^4_0}\right)\pi(\sigma^2)d\sigma^2\notag\\
&\qquad+\int_{\exp(-2\sqrt{\beta n})}^{\exp(2\sqrt{\beta n})}2\exp\left(-n\frac{\kappa_1\sigma^2}{4c_0\sigma^2_0}\right)\pi(\sigma^2)d\sigma^2+2\pi(\mathcal G^c_n)\notag\\
&=\int_{\exp(-2\sqrt{\beta n})}^{\exp(2\sqrt{\beta n})}2\exp\left(-n\frac{\kappa^2_1u^{-2}}{16c_0\sigma^4_0}\right)\pi(u^{-1})u^{-2}du\notag\\
&\qquad+\int_{\exp(-2\sqrt{\beta n})}^{\exp(2\sqrt{\beta n})}2\exp\left(-n\frac{\kappa_1u^{-1}}{4c_0\sigma^2_0}\right)\pi(u^{-1})u^{-2}du+2\pi(\mathcal G^c_n).
\label{eq:s5_8_int}
\end{align}

Let us first consider the first term of (\ref{eq:s5_8_int}). Note that the prior $\pi\left(u^{-1}\right)u^{-2}$ is such that large values of $u$ receive
small probabilities. Hence, if this prior is replaced by an appropriate function which has a thicker tail than the prior, then the resultant integral provides an upper bound
for the first term of (\ref{eq:s5_8_int}). We consider a function 
%Note that for priors with very thick tails the above method with $\tilde\pi(u)$ of the above form need not be suitable. In such cases we let 
$\tilde\pi(u)$ which is of mixture form depending upon $n$, that is, 
we let $\tilde\pi_n(u)=c_3\sum_{r=1}^{M_n}\psi^{\zeta_{rn}}_{rn}\exp(-\psi_{rn} u^2)u^{2(\zeta_{rn}-1)}$, 
where %$B_n=\left[\exp\left(-2\sqrt{\beta n}\right),\exp\left(2\sqrt{\beta n}\right)\right]$, 
$M_n\leq\exp(\sqrt{\beta n})$ is the number of mixture components, $c_3>0$,  
for $r=1,\ldots,M_n$, $\frac{1}{2}<\zeta_{rn}\leq c_4n^q$, for $0<q<1/2$ and $n\geq 1$, where $c_4>0$, and $0<\psi_1\leq\psi_{rn}<c_5<\infty$, for all $r$ and $n$. 
In this case, with $C_1=\frac{1}{16c_0\sigma^4_0}$,
\begin{align}
& \int_{\exp(-2\sqrt{\beta n})}^{\exp(2\sqrt{\beta n})}\exp\left(-C_1\kappa^2_1nu^{-2}\right)\pi(u^{-1})u^{-2}du\notag\\
%&\leq C_2\int_{\exp(-2\sqrt{\alpha T})-\sigma^{-2}_0}^{\exp(2\sqrt{\alpha T})-\sigma^{-2}_0}\exp\left[-\left(C_1mu^{-2}+\frac{u^2}{2\sigma^2_1}\right)\right]u^{-2}du.
&\leq c_3\sum_{r=1}^{M_n}\psi^{\zeta_{rn}}_{rn}
\int_{\exp(-2\sqrt{\beta n})}^{\exp(2\sqrt{\beta n})}\exp\left[-\left(C_1\kappa^2_1nu^{-2}+\psi_{rn}u^2\right)\right]\left(u^2\right)^{\zeta_{rn}-1}du.
\label{eq:term1_bound3_1}
\end{align}
Now the $r$-th integrand of (\ref{eq:term1_bound3_1}) is minimized at %$\tilde u=\sigma^2_1\left(\sqrt{1+\frac{2C_1m}{\sigma^2_1}}-1\right)$, 
$\tilde u^2_{rn}= \frac{\zeta_{rn}-1+\sqrt{(\zeta_{rn}-1)^2+4C_1\psi_{rn}\kappa^2_1 n}}{2\psi_{rn}}$, so that for sufficiently large $n$, 
$c_1\kappa_1\sqrt{\frac{n}{\psi_{rn}}}\leq\tilde u^2_{rn}\leq \tilde c_1\kappa_1\sqrt{\frac{n}{\psi_{rn}}}$, for some positive constants $c_1$ and $\tilde c_1$. 
Now, for sufficiently large $n$, we have $\frac{\tilde u^2_{rn}}{\log\tilde u^2_{rn}}\geq\frac{\zeta_{rn}-1}{\psi_{rn}(1-c_2)}$, for $0<c_2<1$.
Hence, for sufficiently large $n$, $C_1\kappa^2_1n\tilde u^{-2}_{rn}+\psi_{rn}\tilde u^2_{rn}-(\zeta_{rn}-1)\log(\tilde u^2_{rn})\geq c_2\psi_1\tilde u^2_{rn}
\geq C_2\kappa_1\sqrt{\psi_{rn} n}$ for some 
positive constant $C_2$. From these and (\ref{eq:term1_bound3_1}) it follows that
\begin{align}
&\int_{\exp(-2\sqrt{\beta n})}^{\exp(2\sqrt{\beta n})}2\exp\left(-n\frac{\kappa^2_1u^{-2}}{16c_0\sigma^4_0}\right)\pi(u^{-1})u^{-2}du\notag\\
&=c_3\sum_{r=1}^{M_n}\psi^{\zeta_{rn}}_{rn}
\int_{\exp(-2\sqrt{\beta n})}^{\exp(2\sqrt{\beta n})}\exp\left[-\left(C_1\kappa^2_1nu^{-2}+\psi_1u^2\right)\right]\left(u^2\right)^{\zeta_{rn}-1}du\notag\\
&\leq c_3M_n\exp\left[-\left(C_2\kappa_1\sqrt{n\psi_1}-2\sqrt{\beta n}-\tilde c_5 n^q\right)\right]\notag\\
&\leq c_3\exp\left[-\left(C_2\kappa_1\sqrt{n\psi_1}-3\sqrt{\beta n}-\tilde c_5 n^q\right)\right].
\label{eq:term1_bound3_2}
\end{align}
for some constant $\tilde c_5$. 
Since $\kappa_1$ is as large as desired, $C_2\kappa_1\sqrt{n\psi_1}-3\sqrt{\beta n}-\tilde c_5 n^q>0$ for large enough $n$.

For the second term of (\ref{eq:s5_8_int}), we consider $\tilde\pi_n(u)=c_3\sum_{r=1}^{M_n}\psi^{\zeta_{rn}}_{rn}\exp(-\psi_{rn} u)u^{(\zeta_{rn}-1)}$, with
$M_n\leq\exp(\sqrt{\beta n})$ is the number of mixture components, $c_3>0$, for $r=1,\ldots,M_n$, $0<\zeta_{rn}\leq c_4n^q$, for $0<q<1/2$ and $n\geq 1$, 
where $c_4>0$, and $0<\psi_1\leq\psi_{rn}<c_5<\infty$, for all $r$ and $n$. Thus, the only difference here with the previous definition of $\tilde\pi_n(u)$
is that here $\zeta_{rn}>0$ instead of $\zeta_{rn}>\frac{1}{2}$, which is due to the fact that here $u^2$ is replaced with $u$. In the same way as in (\ref{eq:term1_bound3_2}), it then
follows that
\begin{equation}
\int_{\exp(-2\sqrt{\beta n})}^{\exp(2\sqrt{\beta n})}2\exp\left(-n\frac{\kappa_1u^{-1}}{4c_0\sigma^2_0}\right)\pi(u^{-1})u^{-2}du
\leq c_3\exp\left[-\left(C_2\sqrt{\kappa_1n\psi_1}-3\sqrt{\beta n}-\tilde c_5 n^q\right)\right].
\label{eq:term1_bound3_3}
\end{equation}
Again, $C_2\sqrt{\kappa_1n\psi_1}-3\sqrt{\beta n}-\tilde c_5 n^q>0$ for sufficiently large $n$.

%The third term of the right hand side of (\ref{eq:s5_6}) is the probability of a deterministic quantity with respect to the distribution of $\by_n$, and is zero for large enough 
%$n$ due to (\ref{eq:slln1}). In other words, there exists $n_0\geq 1$ such that for $n\geq n_0$,
%\begin{equation}
%P\left(\left|\frac{1}{2\sigma^2}\times\frac{1}{n}\sum_{i=1}^n\left(\eta(\bx_i)-\eta_0(\bx_i)\right)^2
%-\frac{1}{2\sigma^2}E_{\bX}\left(\eta(\bX)-\eta_0(\bX)\right)^2\right|>\frac{\kappa_1}{4}\right)=0.
%\label{eq:zero_prob}
%\end{equation}
%In the case of random covariates $\bX$, it can be proved in the same way as (\ref{eq:bound_reference}), using the fact that 
%$\underset{\bx\in\mathcal X}{\sup}~\left(\eta(\bx)-\eta_0(\bx)\right)^2 \leq \|\eta-\eta_0\|^2$, that 
%\begin{equation}
%P\left(\left|\frac{1}{2\sigma^2}\times\frac{1}{n}\sum_{i=1}^n\left(\eta(\bx_i)-\eta_0(\bx_i)\right)^2
%-\frac{1}{2\sigma^2}E_{\bX}\left(\eta(\bX)-\eta_0(\bX)\right)^2\right|>\frac{\delta}{4}\right)
%=O\left(n^{-3}\right).
%\label{eq:zero_prob2}
%\end{equation}
For the third term, let us first consider the case of random covariates $\bX$. Here observe that by Hoeffding's inequality (\ctn{Hoeffding63}),
\begin{align}
&P\left(\left|\frac{1}{2\sigma^2}\times\frac{1}{n}\sum_{i=1}^n\left(\eta(\bx_i)-\eta_0(\bx_i)\right)^2
-\frac{1}{2\sigma^2}E_{\bX}\left(\eta(\bX)-\eta_0(\bX)\right)^2\right|>\frac{\kappa_1}{4}\right)\notag\\
&\qquad\leq \exp\left\{-\frac{n^2\kappa^2_1\sigma^4}{144n\|\eta-\eta_0\|^2}\right\}=\exp\left\{-\frac{n\kappa^2_1\sigma^4}{144\|\eta-\eta_0\|^2}\right\},
\label{eq:zero_prob2}
\end{align}
where $\|\eta-\eta_0\|$ is clearly the upper bound of $|\eta(\cdot)-\eta_0(\cdot)|$. Such an upper bound is finite since $\mathcal X$ is compact, $\eta(\cdot)$ is continuous on $\mathcal X$,
and $\|\eta_0\|<\infty$. The same inequality holds when the covariates are non-random; here we can view $\varphi(\bx_i)$; $i=1,\ldots,n$, as a set of independent realizations
from some independent stochastic process.

It follows that
\begin{align}
&\int_{\mathcal S^c}P\left(\left|\frac{1}{2\sigma^2}\times\frac{1}{n}\sum_{i=1}^n\left(\eta(\bx_i)-\eta_0(\bx_i)\right)^2
-\frac{1}{2\sigma^2}E_{\bX}\left(\eta(\bX)-\eta_0(\bX)\right)^2\right|>\frac{\kappa_1}{4}\right)d\pi(\theta)\notag\\
&\leq\int_{\mathcal G_n}\exp\left\{-\frac{n\kappa^2_1\sigma^4}{144\|\eta-\eta_0\|^2}\right\}d\pi(\theta)+\pi(\mathcal G^c_n)\notag\\
&=\int_{\|\eta\|\leq\exp(\sqrt{\beta n})}\|\eta-\eta_0\|\left[\int_{\|\eta-\eta_0\|\exp(-2\sqrt{\beta n})}^{\|\eta-\eta_0\|\exp(2\sqrt{\beta n})}
\exp\left(-\frac{n\kappa^2_1u^{-2}}{144}\right)\pi\left(\frac{\|\eta-\eta_0\|}{u}\right)u^{-2}du\right]\pi\left(\|\eta\|\right)d\|\eta\|\notag\\
&\qquad+\pi(\mathcal G^c_n).
\label{eq:zero_prob3}
\end{align}

Since $\pi\left(\sigma^2>\exp(2\sqrt{\beta n})\right)\leq \exp(-\beta n)$, it is evident that small values of $u$ receive little mass with respect to %much the mass of 
$\pi\left(\frac{\|\eta-\eta_0\|}{u}\right)u^{-2}$. %is concentrated around zero, where the function
%However, the function $\exp\left(-\frac{n\kappa^2_1u^{-2}}{144}\right)$ is large for small values of $u$, so that the first term of (\ref{eq:zero_prob3}) is relatively small.
%$\exp\left(-C_{11}nu^{-2}\right)$ is small. 
%To give greater weight to the function, we can replace 
To obtain an upper bound to the first term of (\ref{eq:zero_prob3}), as before we replace
$\pi\left(\frac{\|\eta-\eta_0\|}{u}\right)u^{-2}$
with a thick-tailed mixture function of the form $\tilde\pi_{\eta,n}(u)
=c_3\sum_{r=1}^{M_n}\|\eta-\eta_0\|^{\zeta_{rn}}\psi^{\zeta_{rn}}_{rn}\exp\left(-u^2\psi_{rn}\|\eta-\eta_0\|\right)\left(u^2\right)^{(\zeta_{rn}-1)}$, 
for positive constants $0<\psi_2\leq\psi_{rn}<c_5<\infty$ and $\frac{1}{2}<\zeta_{rn}<c_4n^q$. 
%Here $$B_{n,\rho^2}=\left[\rho^2\exp(-2\sqrt{\alpha n})-\frac{\rho^2_0}{\sigma^2_0}, \rho^2\exp(2\sqrt{\alpha n})-\frac{\rho^2_0}{\sigma^2_0}\right].$$
Note that for large values of $\|\eta-\eta_0\|$, $\pi\left(\frac{\|\eta-\eta_0\|}{u}\right)u^{-2}$ is small. %large, and small for large $\rho^2$.
This property is broadly inherited by $\tilde\pi_{\eta,n}$, while the tuning parameters $\psi_{rn}$ and $\zeta_{rn}$ can be adjusted to give prior weight to regions far away from zero.
However in $\tilde\pi_{\eta,n}(u)$, note that for $\|\eta-\eta_0\|\geq 1$, $\exp\left(-u^2\psi_{rn}\|\eta-\eta_0\|\right)\leq \exp\left(-u^2\psi_{rn}\right)$, while for $\|\eta-\eta_0\|<1$, 
%the integral of the first term of (\ref{eq:zero_prob3}) must be
%small thanks to multiplication of the range of the integral and the integral itself with $\|\eta-\eta_0\|$. 
the domain of the function $\pi\left(\frac{\|\eta-\eta_0\|}{u}\right)$ is dominated by $u^{-1}$, which is independent of $\eta$.
Hence, for small $\|\eta-\eta_0\|$ 
it suffices to consider a mixture of $\psi^{\zeta_{rn}}_{rn}\exp\left(-u^2\psi_{rn}\right)\left(u^2\right)^{(\zeta_{rn}-1)}$.
%(or a mixture of $M_T$ such terms with different values of $\tilde\psi_6$ and $\tilde\zeta_6$ depending upon $T$) instead of $\exp\left(-u^2\psi_6\rho^2\right)$.
In other words, for all values of $\|\eta-\eta_0\|$, it is sufficient to consider 
$\tilde\pi_n(u)=c_3\sum_{r=1}^{M_n}\psi^{\zeta_{rn}}_{rn}\exp\left(-u^2\psi_{rn}\right)\left(u^2\right)^{(\zeta_{rn}-1)}$.
Hence, up to some positive constant,
\begin{align}
&\int_{\|\eta-\eta_0\|\exp(-2\sqrt{\beta n})}^{\|\eta-\eta_0\|\exp(2\sqrt{\beta n})}\exp\left(-\frac{\kappa^2_1nu^{-2}}{144}\right)
\pi\left(\frac{\|\eta-\eta_0\|}{u}\right)u^{-2}du\notag\\
&\leq \sum_{r=1}^{M_n}\psi^{\zeta_{rn}}_{rn}
\int_{\|\eta-\eta_0\|\exp(-2\sqrt{\beta n})}^{\|\eta-\eta_0\|\exp(2\sqrt{\beta n})}
\exp\left[-\left(\frac{\kappa^2_1nu^{-2}}{144}+\psi_{rn}u^2-(\zeta_{rn}-1)\log u^2\right)\right]du.
\label{eq:root1}
\end{align}
The term within the parenthesis in the exponent of (\ref{eq:root1}) is minimized at $\tilde u^2_{rn}=\frac{\zeta_{rn}-1+\sqrt{(\zeta_{rn}-1)^2+\frac{\psi_{rn}\kappa^2_1n}{36}}}{2\psi_{rn}}$.
Note that $\tilde C_{01}\kappa_1\sqrt{\frac{n}{\psi_{rn}}}\leq\tilde u^2_{rn}\leq\tilde C_{11}\kappa_1\sqrt{\frac{n}{\psi_{rn}}}$, for large enough $n$, for positive constants
$\tilde C_{01}$ and $\tilde C_{11}$. Hence, for large $n$, the 
term within the parenthesis in the exponent of (\ref{eq:root1}) exceeds $\psi_{rn}\tilde u^2\geq \tilde C_{02}\times\kappa_1\sqrt{\psi_{rn} n}$, for $\tilde C_{02}>0$.
Thus, (\ref{eq:root1}) is bounded above by a constant times $\|\eta-\eta_0\|\exp\left(-\tilde C_{02}\times\kappa_1\sqrt{\psi_2 n}+3\sqrt{\beta n}+\tilde c_5 n^q\right)$.
Hence, %the first term of (\ref{eq:zero_prob3}) is bounded above by 
\begin{align}
&\int_{\mathcal S^c}P\left(\left|\frac{1}{2\sigma^2}\times\frac{1}{n}\sum_{i=1}^n\left(\eta(\bx_i)-\eta_0(\bx_i)\right)^2
-\frac{1}{2\sigma^2}E_{\bX}\left(\eta(\bX)-\eta_0(\bX)\right)^2\right|>\frac{\kappa_1}{4}\right)d\pi(\theta)\notag\\
&\qquad\leq 4\exp\left(-\tilde C_{02}\times\kappa_1\sqrt{\psi_2 n}+5\sqrt{\beta n}+\tilde c_5 n^q\right)+\pi\left(\mathcal G^c_n\right).
\label{eq:zero_prob4}
\end{align}
Since $\kappa_1$ is as large as desired, the exponent is negative.

For the fourth term, note that 
$$
Z_n=\frac{1}{n}\sum_{i=1}^n\left(\frac{y_i-\eta_0(\bx_i)}{\sigma_0}\right)\left(\eta(\bx_i)-\eta_0(\bx_i)\right) 
\sim N\left(0,\frac{1}{n^2}\sum_{i=1}^n\left(\eta(\bx_i)-\eta_0(\bx_i)\right)\right).$$
Then since
$$\sum_{i=1}^n\left(\eta(\bx_i)-\eta_0(\bx_i)\right)^2
\leq n\left(\underset{\bx\in\mathcal X}{\sup}~|\eta(\bx)-\eta_0(\bx)|\right)^2=n\|\eta-\eta_0\|^2,$$
\begin{align}
&P\left(\left|\frac{1}{\sigma^2}\times\frac{1}{n}\sum_{i=1}^n\left(y_i-\eta_0(\bx_i)\right)\left(\eta(\bx_i)-\eta_0(\bx_i)\right)\right|>\frac{\kappa_1}{4}\right)
= P\left(\left|Z_n\right|>\frac{\kappa_1\sigma^2}{4\sigma_0}\right)\notag\\
&\ \ \leq 2\exp\left(-\frac{n\kappa^2_1\sigma^4}{32\sigma^2_0\|\eta-\eta_0\|^2}\right).
%&\ \ \leq E\left(Z^6_n\right)\left(\frac{4\sigma_0}{\delta\sigma^2}\right)^6
%=15n^{-6}\left(\frac{4\sigma_0}{\delta\sigma^2}\right)^6\left[\sum_{i=1}^n(\eta(\bx_i)-\eta_0(\bx_i))^2\right]^3\notag\\
%&\ \ \leq 15n^{-3}\left(\frac{4\sigma_0}{\delta}\right)^6\left(\frac{\|\eta-\eta_0\|}{\sigma^2}\right)^6.
%%&\ \ \leq 15n^{-3}\left(\frac{4\sigma_0}{\delta}\right)^6\left(\frac{\kappa_0}{\xi^2}+\frac{1}{\xi\kappa_1}\right)^6. 
\label{eq:s5_9}
\end{align}
Hence, in the same way as (\ref{eq:zero_prob4}), we obtain
\begin{align}
&\int_{\mathcal S^c}P\left(\left|\frac{1}{\sigma^2}\times\frac{1}{n}\sum_{i=1}^n\left(y_i-\eta_0(\bx_i)\right)
\left(\eta(\bx_i)-\eta_0(\bx_i)\right)\right|>\frac{\kappa_1}{4}\right)d\pi(\theta)\notag\\
&\leq \int_{\mathcal G_n}2\exp\left(-\frac{n\kappa^2_1\sigma^4}{32\sigma^2_0\|\eta-\eta_0\|^2}\right)d\pi(\theta)+2\pi\left(\mathcal G^c_n\right)\notag\\
&\leq 4\exp\left(-\tilde C_{03}\times\kappa_1\sqrt{\psi_3 n}+5\sqrt{\beta n}+\tilde c_5 n^q\right)+2\pi\left(\mathcal G^c_n\right),
\label{eq:zero_prob5}
\end{align}
for some positive constant $\tilde C_{03}$. As in (\ref{eq:zero_prob3}), the exponent is negative.

Combining (\ref{eq:s5_6}), (\ref{eq:s5_7_int}), (\ref{eq:s5_8_int}), (\ref{eq:term1_bound3_2}), (\ref{eq:term1_bound3_3}), (\ref{eq:zero_prob3}), (\ref{eq:zero_prob4}), (\ref{eq:zero_prob5}),
and noting that $\sum_{n=1}^{\infty}\pi\left(\mathcal G^c_n\right)<\sum_{n=1}^{\infty}\alpha\exp\left(-\beta n\right)<\infty$, we obtain
\begin{equation*}
\int_{\mathcal S^c}P\left(\left|\frac{1}{n}\log R_n(\theta)+h(\theta)\right|>\kappa_1\right)d\pi(\theta)<\infty.
\end{equation*}

\subsection{Verification of (S7)}
\label{subsec:S7}
For any set $A$ such that $\pi(A)>0$, $\mathcal G_n\cap A\uparrow A$. It follows from this and continuity of $h$ that $h\left(\mathcal G_n\cap A\right)\downarrow h\left(A\right)$ as
$n\rightarrow\infty$, so that (S7) holds.

%Thus, all the assumptions (S1)--(S7) are satisfied, showing that Theorems \ref{theorem:shalizi1} and \ref{theorem:shalizi2} hold.
%Formally, we have the following theorem.
%\begin{theorem}
%\label{theorem:gp1}
%Assume the Gaussian process model given by (\ref{eq:model1}), (\ref{eq:model2}), (\ref{eq:gp1}) and (\ref{eq:prior_sigma}). Then under the conditions (A1) -- (A5),
%(\ref{eq:supp_post_conv1}) holds. 
%Also, for any measurable set $A$ with $\pi(A)>0$, if $\beta>2h(A)$, where $h$ is given by (\ref{eq:h}), or if $A\subset\cap_{k=n}^{\infty}\mathcal G_k$ for some $n$, 
%where $\mathcal G_k$ is given by (\ref{eq:G}), then
%(\ref{eq:post_conv2}) holds.
%\end{theorem}

\section{Verification of Shalizi's conditions for Gaussian process regression with double exponential error distribution}
\label{sec:de}

%We now assume the same set-up as (\ref{eq:model1}), (\ref{eq:gp1}) and (\ref{eq:prior_sigma}), but assume that $\epsilon_i\stackrel{iid}{\sim}DE(0,\sigma)$, where
%$DE(0,\sigma)$ stands for the double exponential distribution with median $0$ and scale parameter $\sigma$ with density 
%\begin{equation}
%f(\epsilon)=\frac{1}{2\sigma}\exp\left(-\frac{|\epsilon|}{\sigma}\right);~\epsilon\in\mathbb R.
%\label{eq:de1}
%\end{equation}

%\begin{align}
%y_i&=\eta(\bx_i)+\epsilon_i;~i=1,\ldots,n;\label{eq:model1}\\
%\epsilon_i &\stackrel{iid}{\sim}N\left(0,\sigma^2\right);\label{eq:model2}\\
%\eta(\cdot) &\sim GP\left(\mu(\cdot),c(\cdot,\cdot)\right);\label{eq:gp1}\\
%\sigma &\sim\pi_{\sigma}(\cdot).
%\label{eq:prior_sigma}
%\end{align}

\subsection{Verification of (S1)}
\label{subsec:S1_de}
In this case,
\begin{equation}
\frac{1}{n}\log R_n(\theta)=\log\left(\frac{\sigma_0}{\sigma}\right)+\frac{1}{\sigma_0}\times\frac{1}{n}\sum_{i=1}^n\left|y_i-\eta_0(\bx_i)\right)|
-\frac{1}{\sigma}\times\frac{1}{n}\sum_{i=1}^n\left|y_i-\eta(\bx_i)\right|.
\label{eq:R_de}
\end{equation}
%We show that the right hand side of (\ref{eq:R1}), which we denote as $f(\by_n,\theta)$, is continuous in $(\by_n,\theta)$, which is sufficient to confirm measurability of $R_n(\theta)$.
%Let $\|(\by_n,\theta)\|=\|\by_n\|+\|\theta\|$, where $\|\by_n\|$ is the Euclidean norm and $\|\theta\|=\|\eta\|+|\sigma|$, with
%$\|\eta\|=\underset{\bx\in\mathcal X}{\sup}~|\eta(\bx)|$. Since $\mathcal X$ is compact and $\eta$ is almost surely continuous, it follows that $\|\eta\|<\infty$ almost surely.
%
%Consider $\by_{1n}=(y_{11},y_{12},\ldots,y_{1n})^T$, $\by_{2n}=(y_{21},y_{22},\ldots,y_{2n})^T$, $\theta_1$ and $\theta_2$ 
%such that, given $\varepsilon>0$, $\|(\by_{1n},\theta_1)-(\by_{2n},\theta_2)\|<\frac{\varepsilon}{c}$, for some finite $c>0$.
%Letting $\boeta_{0n}=(\eta_0(\bx_1),\ldots,\eta_0(\bx_n))^T$, observe that
As before, note that
\begin{align}
&\Bigg|\frac{1}{n}\sum_{i=1}^n\left|y_{1i}-\eta_0(\bx_i)\right|-\frac{1}{n}\sum_{i=1}^n\left|y_{2i}-\eta_0(\bx_i)\right|\Bigg |\notag\\
&\leq\frac{1}{n}\sum_{i=1}^n\Bigg |\left|y_{1i}-\eta_0(\bx_i)\right|-\left|y_{2i}-\eta_0(\bx_i)\right|\Bigg |\notag\\
&\leq\frac{1}{n}\sum_{i=1}^n|y_{1i}-y_{2i}|\notag\\
&\leq n^{-\frac{1}{2}}\sqrt{\sum_{i=1}^n(y_{1i}-y_{2i})^2}\notag\\
&=n^{-\frac{1}{2}}\|\by_{1n}-\by_{2n}\|,\notag
%&\ \ \leq\|\by_{1n}-\by_{2n}\|\times\left(\frac{\|\by_{1n}-\boeta_{0n}\|}{n}+\frac{\|\by_{2n}-\boeta_{0n}\|}{n}\right).
%\label{eq:cont3}
\end{align}
from which Lipschitz continuity follows.
Similarly, 
\begin{align}
&\Bigg|\frac{1}{n}\sum_{i=1}^n\left|y_{1i}-\eta_1(\bx_i)\right|-\frac{1}{n}\sum_{i=1}^n\left|y_{2i}-\eta_2(\bx_i)\right|\Bigg |\notag\\ 
&\leq\frac{1}{n}\sum_{i=1}^n\left|y_{1i}-\eta_1(\bx_i)-y_{2i}+\eta_2(\bx_i)\right|\notag\\
&\leq\frac{1}{n}\sum_{i=1}^n\left[\left|y_{1i}-y_{2i}\right|+\left|\eta_1(\bx_i)-\eta_2(\bx_i)\right|\right]\notag\\
&\leq n^{-\frac{1}{2}}\|\by_1-\by_2\|+\|\eta_1-\eta_2\|,
\label{eq:lipcont_de}
\end{align}
which implies continuity of $\frac{1}{n}\sum_{i=1}^n\left|y_i-\eta(\bx_i)\right|$ with respect to $\by$ and $\eta$.
In other words, (\ref{eq:R2}) is continuous and hence measurable, as before. Measurability, when the covariates are considered random, also follows as before,
using measurability of $\eta_0(\bX)$ as assumed in (A4).

\subsection{Verification of (S2) and proof of Lemma \ref{lemma:lemma1} for double-exponential errors}
\label{subsec:S2_de}
Now note that if $\epsilon_i=y_i-\eta_0(\bx_i)$ has the double exponential density of the form 
\begin{equation*}
f(\epsilon)=\frac{1}{2\sigma}\exp\left(-\frac{|\epsilon|}{\sigma}\right);~\epsilon\in\mathbb R.
%\label{eq:de1}
\end{equation*}
with $\sigma$ replaced with $\sigma_0$, then
\begin{align}
&E_{\theta_0}\left|y_i-\eta_0(\bx_i)\right|=\sigma_0;\label{eq:de_exp1}\\ 
&E_{\theta_0}\left|y_i-\eta(\bx_i)\right|=E_{\theta_0}\left|(y_i-\eta_0(\bx_i))+(\eta_0(\bx_i)-\eta(\bx_i))\right|\notag\\
&\qquad\qquad\qquad\quad=|\eta_0(\bx_i)-\eta(\bx_i)|+\sigma_0\exp\left(-\frac{|\eta_0(\bx_i)-\eta(\bx_i)|}{\sigma_0}\right).
\label{eq:de_exp2}
\end{align}
It follows from (\ref{eq:de_exp1}), (\ref{eq:de_exp2}) and (A3), that
\begin{align}
&\frac{1}{n}\sum_{i=1}^nE_{\theta_0}\left|y_i-\eta_0(\bx_i)\right|=\sigma_0;\label{eq:de_exp3}\\
&\frac{1}{n}\sum_{i=1}^nE_{\theta_0}\left|y_i-\eta(\bx_i)\right|=
\frac{1}{n}\sum_{i=1}^n\left[|\eta(\bx_i)-\eta_0(\bx_i)|+\sigma_0\exp\left(-\frac{|\eta(\bx_i)-\eta_0(\bx_i)|}{\sigma_0}\right)\right]\notag\\
&\ \ \rightarrow E_{\bX}\left|\eta(\bX)-\eta_0(\bX)\right|+\sigma_0E_{\bX}\left[\exp\left(-\frac{|\eta(\bX)-\eta_0(\bX)|}{\sigma_0}\right)\right],
~\mbox{as}~n\rightarrow\infty.\label{eq:de_exp4}
\end{align}
Using (\ref{eq:de_exp3}) and (\ref{eq:de_exp4}) we see that as $n\rightarrow\infty$,
\begin{align}
&\frac{1}{n}E_{\theta_0}\left[\log R_n(\theta)\right]=\log\left(\frac{\sigma_0}{\sigma}\right)
+\frac{1}{\sigma_0}\times\frac{1}{n}\sum_{i=1}^nE_{\theta_0}\left|y_i-\eta_0(\bx_i)\right|
-\frac{1}{\sigma}\times\frac{1}{n}\sum_{i=1}^nE_{\theta_0}\left|y_i-\eta(\bx_i)\right|\notag\\
&\rightarrow\log\left(\frac{\sigma_0}{\sigma}\right)+1-\frac{1}{\sigma}E_{\bX}\left|\eta(\bX)-\eta_0(\bX)\right|
-\frac{\sigma_0}{\sigma}E_{\bX}\left[\exp\left(-\frac{|\eta(\bX)-\eta_0(\bX)|}{\sigma_0}\right)\right],\notag\\
&\ \ =-h(\theta),
\label{eq:R_de2}
\end{align}
where
\begin{equation*}
h(\theta)=\log\left(\frac{\sigma}{\sigma_0}\right)-1+\frac{1}{\sigma}E_{\bX}\left|\eta(\bX)-\eta_0(\bX)\right|
+\frac{\sigma_0}{\sigma}E_{\bX}\left[\exp\left(-\frac{|\eta(\bX)-\eta_0(\bX)|}{\sigma_0}\right)\right].
%\label{eq:h_de}
\end{equation*}
As in the case of Gaussian errors, the results remain the same if the covariates are assumed to be random.

\subsection{Verification of (S3) and proof of Theorem \ref{theorem:theorem1} for double exponential errors}
\label{subsec:S3_de}
We now show that for all $\theta\in\Theta$, $\underset{n\rightarrow\infty}{\lim}\frac{1}{n}\log R_n(\theta)=-h(\theta)$, almost surely.
First note that 
\begin{align}
&\left|\frac{1}{n}R_n(\theta)+h(\theta)\right|\leq\left|\frac{1}{n}\sum_{i=1}^n\frac{|y_i-\eta_0(\bx_i)|}{\sigma_0}-1\right|\notag\\
&\quad+\left|\frac{1}{n}\sum_{i=1}^n\frac{|y_i-\eta(\bx_i)|}{\sigma}-\frac{1}{\sigma}E_{\bX}\left|\eta(\bX)-\eta_0(\bX)\right|-
\frac{\sigma_0}{\sigma}E_{\bX}\left[\exp\left(-\frac{|\eta(\bX)-\eta_0(\bX)|}{\sigma_0}\right)\right]\right|.
\label{eq:h_de2}
\end{align}
Since $\frac{|y_i-\eta_0(\bx_i)|}{\sigma_0}$ has the exponential distribution with mean one, the term 
$\left|\frac{1}{n}\sum_{i=1}^n\frac{|y_i-\eta_0(\bx_i)|}{\sigma_0}-1\right|\rightarrow 0$ almost surely as $n\rightarrow\infty$ by the
strong law of large numbers.
That the term (\ref{eq:h_de2}) also tends to zero almost surely as $n\rightarrow\infty$ can be shown using the Borel-Cantelli lemma, using the inequality
(\ref{eq:bound3}), and replacing $\kappa_1$ in that inequality with any $\delta_1>0$.
In other words, it holds that for all $\theta\in\Theta$, $\underset{n\rightarrow\infty}{\lim}\frac{1}{n}\log R_n(\theta)=-h(\theta)$, almost surely.
Also, it follows from (\ref{eq:R_de}), (\ref{eq:lipcont_de}), (\ref{eq:h_de}), Lipschitz continuity of $x\mapsto\exp(-|x|)$, boundedness of the first derivative with respect to $\sigma$, 
that $\frac{1}{n}\log R_n(\theta)+h(\theta)$ is Lipschitz on $\theta\in\mathcal G_n\setminus I=\mathcal G_n$, which is compact. 
%Also, it is straightforward to directly verify, using the same techniques as (\ref{eq:lipcont_de}), that $\frac{1}{n}\log R_n(\theta)+h(\theta)$ is Lipschitz with respect to $\eta$.
%Since the function $\frac{1}{n}\log R_n(\theta)+h(\theta)$ is also differentiable in $\sigma$, which is bounded in any $\mathcal G\in\left\{\mathcal G_1,\mathcal G_2,\ldots,\right\}$,
As a result, it follows that $\frac{1}{n}\log R_n(\theta)+h(\theta)$ is stochastically equicontinuous in $\mathcal G\in\left\{\mathcal G_1,\mathcal G_2,\ldots,\right\}$. Hence, the convergence  
$\underset{n\rightarrow\infty}{\lim}\frac{1}{n}\log R_n(\theta)=-h(\theta)$ occurs uniformly for $\theta\in\mathcal G$, almost surely.

\subsection{Verification of (S4)}
\label{subsec:S4_de}
Note that $h(\theta)\leq\log\left(\frac{\sigma}{\sigma_0}\right)-1+\frac{\|\eta-\eta_0\|+\sigma_0}{\sigma}$. Now $0<\|\eta-\eta_0\|<\infty$ and 
$0<\sigma<\infty$ with prior probability one. Consequently, it follows that
$h(\theta)<\infty$ with probability one, so that $I=\emptyset$ and hence, $\mathcal G_n\setminus I=\mathcal G_n$.

\subsection{Verification of (S5)}
\label{subsec:S5_de}

Verification of (S5) (1) and (S5) (2) remains the same as for Gaussian noise. (S5) (3) follows in the same way as for Gaussian noise is we can show that
$h(\theta)$ is continuous in $\theta$.
To see that $h(\theta)$ is continuous in $\theta$, again assume that $\eta_j\rightarrow\tilde\eta$ as $j\rightarrow\infty$ in the sense that $\|\eta_j-\tilde\eta\|\rightarrow 0$
as $j\rightarrow\infty$. Then $\left|E_{\bX}\left|\eta_j(\bX)-\eta_0(\bX)\right|-E_{\bX}\left|\tilde\eta(\bX)-\eta_0(\bX)\right|\right|\leq E_{\bX}\left|\eta_j(\bX)-\tilde\eta(\bX)\right|
\leq\|\eta_j-\tilde\eta\|\rightarrow 0$ as $j\rightarrow\infty$. Also, 
\begin{align}
&\left|E_{\bX}\left[\exp\left(-\frac{|\eta_j(\bX)-\eta_0(\bX)|}{\sigma_0}\right)\right]-E_{\bX}\left[\exp\left(-\frac{|\tilde\eta(\bX)-\eta_0(\bX)|}{\sigma_0}\right)\right]\right|\notag\\ 
&\leq E_{\bX}\left[\exp\left(-\left|\tilde\eta(\bX)-\eta_0(\bX)\right|\right)\times
\left|\exp\left(-\frac{\left(|\eta_j(\bX)-\eta_0(\bX)|-|\tilde\eta(\bX)-\eta_0(\bX)|\right)}{\sigma_0}\right)-1\right|\right]\notag\\
&\leq E_{\bX}\left[\exp\left(-\left|\tilde\eta(\bX)-\eta_0(\bX)\right|\right)\times
\left|\exp\left(\frac{|\eta_j(\bX)-\tilde\eta(\bX)|}{\sigma_0}\right)-1\right|\right]\notag\\
&\leq \left|\exp\left(\frac{\|\eta_j-\tilde\eta\|}{\sigma_0}\right)-1\right|\times E_{\bX}\left[\exp\left(-\left|\tilde\eta(\bX)-\eta_0(\bX)\right|\right)\right]\notag\\
&\rightarrow 0,~\mbox{as}~j\rightarrow\infty.\notag
\end{align}
Continuity of $h(\theta)$ hence follows easily.

\subsection{Verification of (S6) and proof of Theorem \ref{theorem:theorem3} for double exponential errors}
\label{subsec:S6_de}
It follows from (\ref{eq:h_de2}) that for all $\theta\in\Theta$, for $\kappa_1=\kappa-h(\Theta)$, we have
\begin{align}
&P\left(\left|\frac{1}{n}\log R_n(\theta)+h(\theta)\right|>\kappa_1\right)
\leq P\left(\left|\frac{1}{\sigma_0}\times\frac{1}{n}\sum_{i=1}^n\left|y_i-\eta_0(\bx_i)\right|-1\right|>\frac{\kappa_1}{2}\right)\notag\\
&\qquad+P\left(\left|\frac{1}{\sigma}\times\frac{1}{n}\sum_{i=1}^n\left|y_i-\eta(\bx_i)\right|
-\frac{1}{\sigma}E_{\bX}\left|\eta(\bX)-\eta_0(\bX)\right|\right.\right.\notag\\
&\qquad\qquad\qquad\left.\left.-\frac{\sigma_0}{\sigma}E_{\bX}\left(\exp\left\{-\frac{\left|\eta(\bX)-\eta_0(\bX)\right|}{\sigma_0}\right\}\right)\right|
>\frac{\kappa_1}{2}\right).
\label{eq:unif_de1}
\end{align}

%Now note that $Z_n=\frac{1}{\sigma_0}\sum_{i=1}^n\left|y_i-\eta_0(\bx_i)\right|\sim Gamma(n,1)$, where $Gamma(a,b)$ stands for the gamma distribution with mean $a/b$ and
%variance $a/b^2$. %Using the method of \ctn{Choi07} we obtain the following bound for the first term of the right hand side of (\ref{eq:unif_de1}):
Since $\frac{|y_i-\eta_0(\bx_i)|}{\sigma_0}$ are exponential random variables with expectation one, it follows that $\frac{|y_i-\eta_0(\bx_i)|}{\sigma_0}-1$ are zero-mean, 
independent sub-exponential random variables with some parameter $s>0$. Hence, by Bernstein's inequality (\ctn{Uspensky37}, \ctn{Bennett62}, \ctn{Massart03}),
\begin{align}
&P\left(\left|\frac{1}{\sigma_0}\times\frac{1}{n}\sum_{i=1}^n\left|y_i-\eta_0(\bx_i)\right|-1\right|>\frac{\kappa_1}{2}\right)
\leq 2\exp\left(-\frac{n}{2}\min\left\{\frac{\kappa^2_1}{4s^2},\frac{\kappa_1}{2s}\right\}\right).\notag
%=P\left(Z_n>n\left(1+\frac{\kappa_1}{2}\right)\right)+P\left(Z_n<n\left(1-\frac{\kappa_1}{2}\right)\right)\notag\\
%&\qquad\qquad\leq\exp\left\{-n\left(\frac{\kappa^2_1}{4}-\frac{\kappa^3_1}{6}\right)\right\}+\exp\left(-\frac{n\kappa^2_1}{4}\right).\notag
%\label{eq:gamma_de1}
\end{align}
Hence,
\begin{equation}
\int_{\mathcal S^c}P\left(\left|\frac{1}{\sigma_0}\times\frac{1}{n}\sum_{i=1}^n\left|y_i-\eta_0(\bx_i)\right|-1\right|>\frac{\kappa_1}{2}\right)
\leq 2\exp\left(-\frac{n}{2}\min\left\{\frac{\kappa^2_1}{4s^2},\frac{\kappa_1}{2s}\right\}\right).
\label{eq:summable1}
\end{equation}

%For the second term of the right hand side of (\ref{eq:unif_de1}), we make use of the following result presented in \ctn{Choi07}:
%\begin{lemma}[\ctn{Choi07}]
%\begin{itemize}
%\item[(a)]For every random variable $X$ with unimodal distribution symmetric around 0 and every $c\in\mathbb R$,
%\begin{equation}
%P\left((|X| \leq x\right) \geq P\left(|X + c| \leq x\right),~\forall x>0.
%\label{eq:choi1}
%\end{equation}
%\item[(b)]Let $X_1,\ldots,X_n$ and $Y_1,\ldots,Y_n$ be independent random variables. If
%$P\left(X_i \leq a\right) \leq P\left(Y_i\leq a\right)$,
%then, $\forall c \in\mathbb R$,
%\begin{equation}
%P\left(\sum_{i=1}^nX_i\leq c\right)\leq P\left(\sum_{i=1}^nX_i\leq c\right).
%\label{eq:choi2}
%\end{equation}
%\end{itemize}
%\end{lemma}
Let $\bar\varphi=E_{\bX}\left|\eta(\bX)-\eta_0(\bX)\right|+\sigma_0E_{\bX}\left(\exp\left\{-\frac{\left|\eta(\bX)-\eta_0(\bX)\right|}{\sigma_0}\right\}\right)$. 
%Then using Jensen's inequality, 
%\begin{equation}
%\bar\varphi\geq \sigma_0\left[\frac{E_{\bX}\left|\eta(\bX)-\eta_0(\bX)\right|}{\sigma_0}+\exp\left\{-\frac{E_{\bX}\left|\eta(\bX)-\eta_0(\bX)\right|}{\sigma_0}\right\}\right]\geq \sigma_0.
%\label{eq:jensen1}
%\end{equation}
Also, letting
$\varphi(\bx)=\left|\eta(\bx)-\eta_0(\bx)\right|+\sigma_0\left(\exp\left\{-\frac{\left|\eta(\bx)-\eta_0(\bx)\right|}{\sigma_0}\right\}\right)$, note that
\begin{equation}
\frac{1}{n}\sum_{i=1}^n\varphi(\bx_i)\rightarrow\bar\varphi,~\mbox{as}~n\rightarrow\infty.
\label{eq:varphi1}
\end{equation}
With this, the second term of (\ref{eq:unif_de1}) can be bounded as follows:
\begin{align}
&P\left(\left|\frac{1}{\sigma}\times\frac{1}{n}\sum_{i=1}^n\left|y_i-\eta(\bx_i)\right|-\frac{\bar\varphi}{\sigma}\right|>\frac{\kappa_1}{2}\right)\notag\\
%&\ \ \leq P\left(\left|\frac{1}{n}\sum_{i=1}^n\left|y_i-\eta(\bx_i)\right|-\varphi\right|>\frac{\delta\xi}{2}\right)\notag\\
&\ \ = P\left(\sigma^{-1}\left|\frac{1}{n}\sum_{i=1}^n\left\{\left|y_i-\eta(\bx_i)\right|-\varphi(\bx_i)\right\}+\frac{1}{n}\sum_{i=1}^n\varphi(\bx_i)-\bar\varphi\right|
>\frac{\kappa_1}{2}\right)\notag\\
&\ \ \leq P\left(\sigma^{-1}\left|\frac{1}{n}\sum_{i=1}^n\left\{\left|y_i-\eta(\bx_i)\right|-\varphi(\bx_i)\right\}\right|>\frac{\kappa_1}{4}\right)
+P\left(\sigma^{-1}\left|\frac{1}{n}\sum_{i=1}^n\varphi(\bx_i)-\bar\varphi\right|>\frac{\kappa_1}{4}\right).
\label{eq:bound1}
\end{align}
%Now, due to (\ref{eq:varphi1}), there exists $n_0\geq 1$ such that for $n\geq n_0$, such that 
%\begin{equation}
%P\left(\sigma^{-1}\left|\frac{1}{n}\sum_{i=1}^n\varphi(\bx_i)-\bar\varphi\right|>\frac{\kappa_1}{4}\right)=0~\mbox{for}~n\geq n_0.
%\label{eq:bound2}
%\end{equation}
%In the case of random covariates $\bX$, it can be proved in the same way as (\ref{eq:bound_reference}), using the fact that 
%$\underset{\bx\in\mathcal X}{\sup}~\varphi(\bx) \leq \|\eta-\eta_0\|+\sigma_0$, that 
%$$P\left(\sigma^{-1}\left|\frac{1}{n}\sum_{i=1}^n\varphi(\bx_i)-\bar\varphi\right|>\frac{\delta}{4}\right)=O\left(n^{-3}\right).$$
%
In the case of random or non-random covariates $\bX$, again by Hoeffding's inequality,
\begin{equation}
P\left(\sigma^{-1}\left|\frac{1}{n}\sum_{i=1}^n\varphi(\bx_i)-\bar\varphi\right|>\frac{\kappa_1}{4}\right)
\leq \exp\left\{-\frac{n^2\kappa^2_1\sigma^2}{144nC^2}\right\}=\exp\left\{-\frac{n\kappa^2_1\sigma^2}{144C^2}\right\},
\label{eq:hoeff1}
\end{equation}
where $C>0$ is the upper bound of $|\varphi(\cdot)|$. Again, such an upper bound exists since $\mathcal X$ is compact and $\eta(\cdot)$ is continuous on $\mathcal X$.
%The same will be the bound for non-random covariates.
Application of the same method as proving (\ref{eq:term1_bound3_3}) yields
\begin{equation}
\int_{\mathcal S^c}P\left(\sigma^{-1}\left|\frac{1}{n}\sum_{i=1}^n\varphi(\bx_i)-\bar\varphi\right|>\frac{\kappa_1}{4}\right)\pi(\theta)d\theta
\leq c_3\exp\left[-\left(C_2\sqrt{\kappa_1n\psi_1}-3\sqrt{\beta n}-\tilde c_5n^q\right)\right],
\label{eq:summable2}
\end{equation}
where $\kappa_1$ is large enough to make the exponent of (\ref{eq:summable2}) negative.

For the first term of (\ref{eq:bound1}), let us first prove that $|y_i-\eta(\bx_i)|-\varphi(\bx_i)$ are sub-exponential random variables. Then we can apply Bernstein's
inequality to directly bound the term. %Indeed, straightforward calculation shows that for any $t>0$ such that $\sigma_0t<1$,
We need to show that $E_{\theta_0}\left[\exp\left\{t\left(|y_i-\eta(\bx_i)|\right)-\varphi(\bx_i)\right\}\right]\leq\exp\left(\frac{t^2s^2}{2}\right)$
for $|t|\leq s^{-1}$, for some $s>0$.

\subsection{Case 1: $t\geq 0$, $\eta(\bx_i)-\eta_0(\bx_i)>0$}
\label{subsec:case1}
Direct calculation shows that
\begin{align}
&E_{\theta_0}\left[\exp\left\{t\left(|y_i-\eta(\bx_i)|\right)-\varphi(\bx_i)\right\}\right]\notag\\
&=\exp\left(-t\varphi(\bx_i)\right)\times
\frac{\exp\left\{(\eta(\bx_i)-\eta_0(\bx_i))t\right\}-\exp\left(\frac{\eta_0(\bx_i)-\eta(\bx_i)}{\sigma_0}\right)}{1-\sigma^2_0t^2}\notag\\
&\leq\frac{\exp\left\{t\left(\varphi(\bx_i)+\eta(\bx_i)-\eta_0(\bx_i)\right)\right\}}{1-\sigma^2_0t^2}\notag\\
&\leq \frac{\exp\left\{t\left(2\|\eta-\eta_0\|+\sigma_0\right)\right\}}{1-\sigma^2_0t^2}.
\label{eq:subexp1}
\end{align}
To show that (\ref{eq:subexp1}) is bounded above by $\exp(t^2s^2/2)$, we need to show that 
\begin{equation}
f(t)=\frac{t^2s^2}{2}-2(\|\eta-\eta_0\|+\sigma_0)t+\log(1-\sigma^2_0t^2)\geq 0.
\label{eq:subexp2}
\end{equation}
For $t>0$, it is sufficient to show that 
\begin{equation}
\frac{ts^2}{2}\geq 2(\|\eta-\eta_0\|+\sigma_0)-\frac{\log(1-\sigma^2_0t^2)}{t}.
\label{eq:subexp3}
\end{equation}
Now, $-\frac{\log(1-\sigma^2_0t^2)}{t}\rightarrow 0$, as $t\rightarrow 0$. Hence, for any $\epsilon>0$, there exists $\delta(\epsilon)>0$ such that $t\leq\delta(\epsilon)$
implies $-\frac{\log(1-\sigma^2_0t^2)}{t}<\epsilon$. Let $s\geq\frac{C_1\|\eta-\eta_0\|+C_2}{\delta(\epsilon)}$, where $C_1>0$ and $C_2>0$ are sufficiently large quantities. 
Hence, if $\delta(\epsilon)^2\leq t\leq\delta(\epsilon)$, then (\ref{eq:subexp3}), and hence (\ref{eq:subexp2}), is satisfied. Now, $f(t)$ given by (\ref{eq:subexp2}) is continuous in $t$
and $f(0)=0$. Hence, (\ref{eq:subexp2}) holds even for $0\leq t\leq\delta(\epsilon)^2$. In other words,
\begin{equation}
E_{\theta_0}\left[\exp\left\{t\left(|y_i-\eta(\bx_i)|\right)-\varphi\right\}\right]\leq\exp\left(\frac{t^2s^2}{2}\right),~\mbox{for}~0\leq t\leq s^{-1}
\leq\frac{\delta(\epsilon)}{C_1\|\eta-\eta_0\|+C_2}\leq\delta(\epsilon).
\label{eq:subexp4}
\end{equation}

\subsection{Case 2: $t\geq 0$, $\eta(\bx_i)-\eta_0(\bx_i)<0$}
\label{subsec:case2}
In this case,
\begin{align}
&E_{\theta_0}\left[\exp\left\{t\left(|y_i-\eta(\bx_i)|\right)-\varphi(\bx_i)\right\}\right]\notag\\
&=\exp\left(-t\varphi(\bx_i)\right)\times
\frac{\exp\left\{(\eta_0(\bx_i)-\eta(\bx_i))t\right\}+\sigma_0t\exp\left(\frac{\eta(\bx_i)-\eta_0(\bx_i)}{\sigma_0}\right)}{1-\sigma^2_0t^2}\notag\\
&\leq \exp\left(t\varphi(\bx_i)\right)\times
\frac{2\exp\left\{(\eta_0(\bx_i)-\eta(\bx_i))t\right\}}{1-\sigma^2_0t^2}\notag\\
&\leq\frac{\exp\left\{t\left(\varphi(\bx_i)+(\eta_0(\bx_i)-\eta(\bx_i))\right)\right\}}{\frac{1-\sigma^2_0t^2}{2}}\notag\\
&\leq \frac{\exp\left\{t\left(2\|\eta-\eta_0\|+\sigma_0\right)\right\}}{\frac{1-\sigma^2_0t^2}{2}}.\notag
%\label{eq:subexp5}
\end{align}
As in Section \ref{subsec:case1} it can be seen that (\ref{eq:subexp4}) holds.

\subsection{Case 3: $t\leq 0$, $\eta(\bx_i)-\eta_0(\bx_i)>0$}
\label{subsec:case3}
Here
\begin{align}
&E_{\theta_0}\left[\exp\left\{t\left(|y_i-\eta(\bx_i)|\right)-\varphi(\bx_i)\right\}\right]\notag\\
&=\exp\left(-t\varphi(\bx_i)\right)\times
\frac{\exp\left\{(\eta(\bx_i)-\eta_0(\bx_i))t\right\}-\sigma_0|t|\exp\left(\frac{\eta_0(\bx_i)-\eta(\bx_i)}{\sigma_0}\right)}{1-\sigma^2_0t^2}\notag\\
&\leq \exp\left(-t\varphi(\bx_i)\right)\times
\frac{1}{1-\sigma^2_0t^2}\notag\\
&\leq \frac{\exp\left\{-t\left(\|\eta-\eta_0\|+\sigma_0\right)\right\}}{1-\sigma^2_0t^2}.\notag
%\label{eq:subexp6}
\end{align}
Here we need to have
$|t|\left[\frac{|t|s^2}{2}-\left(\|\eta-\eta_0\|+\sigma_0\right)+\frac{\log(1-\sigma^2_0t^2)}{|t|}\right]>0$. In the same way as before it follows that
\begin{equation}
E_{\theta_0}\left[\exp\left\{t\left(|y_i-\eta(\bx_i)|\right)-\varphi\right\}\right]\leq\exp\left(\frac{t^2s^2}{2}\right),~\mbox{for}~0\leq |t|\leq s^{-1}
\leq\frac{\delta(\epsilon)}{C_1\|\eta-\eta_0\|+C_2}\leq\delta(\epsilon).\notag
\label{eq:subexp7}
\end{equation}

\subsection{Case 4: $t\leq 0$, $\eta(\bx_i)-\eta_0(\bx_i)<0$}
\label{subsec:case4}
In this case,
\begin{align}
&E_{\theta_0}\left[\exp\left\{t\left(|y_i-\eta(\bx_i)|\right)-\varphi(\bx_i)\right\}\right]\notag\\
&=\exp\left(-t\varphi(\bx_i)\right)\times
\frac{\exp\left\{(\eta_0(\bx_i)-\eta(\bx_i))t\right\}-\sigma_0|t|\exp\left(\frac{\eta(\bx_i)-\eta_0(\bx_i)}{\sigma_0}\right)}{1-\sigma^2_0t^2}\notag\\
&\leq \exp\left(-t\varphi(\bx_i)\right)\times
\frac{1}{1-\sigma^2_0t^2}\notag\\
&\leq \frac{\exp\left\{-t\left(\|\eta-\eta_0\|+\sigma_0\right)\right\}}{1-\sigma^2_0t^2}.\notag
%\label{eq:subexp8}
\end{align}
Hence, (\ref{eq:subexp7}) holds.

Hence, for $i=1,\ldots,n$, $|y_i-\eta(\bx_i)|-E\left(|y_i-\eta(\bx_i)|\right)$ are 
zero-mean, independent sub-exponential random variables with parameter $s$. In particular, we can set $s=\frac{C_1\|\eta-\eta_0\|+C_2}{\delta(\epsilon)}$. Hence, by Bernstein's inequality,
\begin{align}
&P\left(\sigma^{-1}\left|\frac{1}{n}\sum_{i=1}^n\left\{\left|y_i-\eta(\bx_i)\right|-\varphi(\bx_i)\right\}\right|>\frac{\kappa_1}{4}\right)\notag\\
&\leq 2\max\left\{P\left(\frac{\sigma^{-1}}{n}\sum_{i=1}^n\left\{\left|y_i-\eta(\bx_i)\right|-\varphi(\bx_i)\right\}>\frac{\kappa_1}{4}\right),
P\left(\frac{\sigma^{-1}}{n}\sum_{i=1}^n\left\{\left|y_i-\eta(\bx_i)\right|-\varphi(\bx_i)\right\}< -\frac{\kappa_1}{4}\right)\right\}\notag\\
&\leq 2\exp\left(-\frac{n}{2}\min\left\{\frac{\kappa^2_1\sigma^2}{16s^2},\frac{\kappa_1\sigma}{4s}\right\}\right)\notag\\
&=2\exp\left(-\frac{n}{2}\min\left\{\frac{\kappa^2_1\delta(\epsilon)^2\sigma^2}{16(C_1\|\eta-\eta_0\|+C_2)^2},\frac{\kappa_1\delta(\epsilon)\sigma}{4(C_1\|\eta-\eta_0\|+C_2)}\right\}\right).
\label{eq:bound3}
\end{align}
Applying the same techniques of proving (\ref{eq:zero_prob4}) and (\ref{eq:zero_prob5}) to (\ref{eq:bound3}), it is easy to see that
\begin{align}
&P\left(\sigma^{-1}\left|\frac{1}{n}\sum_{i=1}^n\left\{\left|y_i-\eta(\bx_i)\right|-\varphi(\bx_i)\right\}\right|>\frac{\kappa_1}{4}\right)\notag\\
&\leq\tilde C_1\exp\left\{-\left(\kappa_1\tilde C_2\sqrt{n\psi_1}-\tilde C_3\sqrt{\beta n}-\tilde C_4 n^q\right)\right\}\notag\\
&\qquad+\tilde C_5\exp\left\{-\left(\tilde C_6\sqrt{\kappa_1n\psi_2}-\tilde C_7\sqrt{\beta n}-\tilde C_8 n^q\right)\right\}+2\pi\left(\mathcal G^c_n\right).
\label{eq:summable3}
\end{align}

Gathering (\ref{eq:summable1}), (\ref{eq:summable2}) and (\ref{eq:summable3}) we see that
for all $\theta\in\Theta$, for any $\delta>0$, and for some $a>0$,
\begin{equation}
\sum_{n=1}^{\infty}\int_{\mathcal S^c}P\left(\left|\frac{1}{n}\log R_n(\theta)+h(\theta)\right|>\delta\right)\pi(\theta)d\theta<\infty.
\label{eq:unif_de2}
\end{equation}
%The proof of uniform convergence of (\ref{eq:uniform_conv_de}) over $\mathcal G_n\setminus I$ as required by (S5) (2) follows from the proof of (\ref{eq:uniform_conv_de}). 
%Indeed, it follows from (\ref{eq:R_de}), (\ref{eq:lipcont_de}), (\ref{eq:h_de}), Lipschitz continuity of $x\mapsto\exp(-|x|)$, boundedness of the first derivative with respect to $\sigma$, 
%that $\frac{1}{n}\log R_n(\theta)+h(\theta)$ is Lipschitz on $\theta\in\mathcal G_n\setminus I=\mathcal G_n$, which is compact. 
%Hence, combined with the proof of (\ref{eq:uniform_conv_de}), these guarantee (S5) (2).
%so that 
%$\underset{\theta\in\mathcal G_n}{\sup}~\left|\frac{1}{n}\log R_n(\theta)+h(\theta)\right|
%=\left|\frac{1}{n}\log R_n(\hat\theta)+h(\hat\theta)\right|$, for some $\hat\theta\in\mathcal G_n$, perhaps depending on the data. Since (\ref{eq:unif_de2}) holds for all $\theta\in\Theta$
%and that the upper bound is independent of $\theta$,
%the same must hold for $\theta=\hat\theta$.

\subsection{Verification of (S7)}
\label{subsec:S7_de}
Verification of (S7) is exactly the same as for Gaussian errors.
